# Supplementary material for: Direction-Aware Offline-to-Online Learning in Linear Contextual Bandits
Source: arXiv:2604.24016 source file (2026-05-07)
Supplement: Supplementary file 1 [file appendix.tex]

\section{Obtaining a shift certificate}
\label{app:shift-certificate}

The offline sample already fixes $(G_{\mathrm{off}},\hat\theta_{\mathrm{off}})$. The certificate only
adds \emph{separate} side information about $\theta_*-\theta^\dagger$, in the same spirit as
bias budgets in MIN-UCB \citep{cheung2024}. The assumption is \textbf{mild} because it does not
require knowing $\theta_*$: it asks only for a plausible envelope around shift, and any
\emph{conservative} choice (larger $\rho$, or a smaller $M_{\mathrm{shift}}$ in the Loewner order so
the ellipsoid $\{\Delta:\|\Delta\|_{M_{\mathrm{shift}}}\le\rho\}$ is guaranteed to contain
$\theta_*-\theta^\dagger$) remains valid. The algorithm then never does worse than ignoring offline
geometry: the pooled width inflates and behavior approaches the SupLinUCB fallback
\citep{chu2011}. In particular a very loose certificate recovers the usual
$\widetilde O(\sqrt{dT})$ rate. It is \textbf{practical} because such envelopes arise routinely:
A/B tests where only a few coordinates (e.g.\ treatment effects) may move, domain expertise on logging
versus live traffic, or a small validation draw from the online population from which one can
estimate per-coordinate spread of $\theta_*-\theta^\dagger$ and take diagonal
$M_{\mathrm{shift}}=\mathrm{diag}(1/\hat\sigma_1^2,\ldots,1/\hat\sigma_d^2)$ with a union-bound
choice of $\rho$ (see Section~\ref{sec:experiments}). When no directional information is available, a
default isotropic choice is $(M_{\mathrm{shift}},\rho)=(I,\rho)$, where $\rho$ is any valid
bound on $\|\theta_*-\theta^\dagger\|_2$; this already matches standard isotropic warm-start modeling
(since then $\|\theta_*-\theta^\dagger\|_{M_{\mathrm{shift}}}=\|\theta_*-\theta^\dagger\|_2$).
Section~\ref{sec:related} positions this assumption relative to prior work.

Beyond the simple diagonal recipe above, realistic constructions of $M_{\mathrm{shift}}$ often come
from side information that is already available before deployment:
\begin{itemize}
\item \textbf{Short shadow-traffic or holdout calibration.} A small online-calibration sample can be
split into time slices or bootstrap replicates. Fitting a parameter on each slice gives shift
proxies $\hat\Delta^{(b)}$, from which one may estimate a covariance $\hat\Sigma_\Delta$ and take
$M_{\mathrm{shift}}=(\hat\Sigma_\Delta+\lambda I)^{-1}$, or just its diagonal if only marginal scales
are trusted.
\item \textbf{Multiple historical environments.} If logs are available from several markets, weeks, or
product versions, one can fit one model per environment and use the empirical covariance of their
deviations from a pooled estimate as a proxy for shift geometry. This naturally yields a diagonal,
block-diagonal, or low-rank-plus-diagonal $M_{\mathrm{shift}}$.
\item \textbf{Feature-group budgets from domain knowledge.} When features split into groups with very
different expected stability, such as static user profile features versus prices, promotions, or
treatment interactions, practitioners can assign one scale $s_g$ per group and set
$M_{\mathrm{shift}}=\sum_g s_g^{-2}P_g$, where $P_g$ projects onto group $g$. This turns qualitative
knowledge about which directions drift into a quantitative certificate.
\item \textbf{Prior randomized experiments.} Repeated A/B tests often reveal that only a few treatment
effect coordinates move materially across launches. The empirical covariance of estimated treatment
effect changes across experiments can therefore be used to build $M_{\mathrm{shift}}$, while the
remaining coordinates receive looser isotropic protection.
\end{itemize}
When only coarse information is trustworthy, one can shrink any estimated matrix toward the identity,
for example $M_{\mathrm{shift}}=(1-\alpha)\hat M+\alpha I$, or keep only its diagonal. Such shrinkage
only enlarges the certificate after a corresponding conservative choice of $\rho$, so the main text's
guarantees continue to apply.

\section{Why an isotropic certificate is too coarse}
\label{app:isotropic-too-coarse}

The main text models shift through a directional certificate
$\|\theta_*-\theta^\dagger\|_{M_{\mathrm{shift}}}\le \rho$. The next theorem explains why replacing
this by a single Euclidean summary $\|\theta_*-\theta^\dagger\|_2\le \rho$ is too coarse if one wants a
nontrivial account of \emph{which} offline directions transfer. Even when the offline data law is
identical across instances, the same valid isotropic certificate can hide very different online
hardness depending on how the shift aligns with regret-relevant directions. The statement below is a
finite-action Bernoulli specialization of the main setup used only as motivation; it is independent
of the main proofs above.

\begin{theorem}[An impossibility result: $\rho$-only certificates cannot identify transferable directions]
\label{thm:rho-only-nonident}
There exist universal constants $c_0,c_1>0$ such that the following holds. Fix any horizon $T\ge 1$,
any baseline $\rho_0 \in (0,1/4]$, and any
\[
0 < \rho \le \min\!\left\{\frac{\rho_0}{4},\, c_0 T^{-1/2}\right\}.
\]
Then there exist three instances of the main setup specialized to Bernoulli rewards in dimension
$3$ with parameter norm bound $S=1$, with the same finite action set of size $K=3$ at every round, sharing the same offline
parameter and hence the same offline data law, such that every instance satisfies the same isotropic
certificate
\[
\norm{\theta_*-\theta^\dagger}_2 \le \rho,
\]
but:
\begin{itemize}
\item[(i)] for the hard family $\mathcal{I}_{\mathrm{bad}}=\{I_+,I_-\}$,
every non-anticipatory policy $\pi$ satisfies
\[
\sup_{I \in \mathcal{I}_{\mathrm{bad}}} \E_I[R_T(\pi)]
\ge
c_1 \frac{\rho^2 T}{\rho_0};
\]
\item[(ii)] for the good instance $I_{\mathrm{good}}$,
the deterministic policy that always plays the same fixed action has zero regret.
\end{itemize}
Consequently, if $S=\Phi(D_{\mathrm{off}})$ is any measurable summary of the offline sample, then
$S$ has the same distribution under the good and hard instances, while the online hardness differs.
In particular, under a $\rho$-only interface no offline-only scalar or functional can fully determine
online hardness.
\end{theorem}

\begin{proof}
Let $e_0,e_1,e_2$ denote the canonical basis of $\R^3$, and set
\[
\bar{\rho} := \frac{\rho}{\sqrt{2}}.
\]
Define the three actions
\[
a_0 := e_1,
\qquad
a_+ := \frac{\rho_0 e_1 + \bar{\rho} e_2}{\sqrt{\rho_0^2+\bar{\rho}^2}},
\qquad
a_- := \frac{\rho_0 e_1 - \bar{\rho} e_2}{\sqrt{\rho_0^2+\bar{\rho}^2}},
\]
and lift them to
\[
x^{(0)} := \frac{e_0+a_0}{\sqrt{2}},
\qquad
x^{(+)} := \frac{e_0+a_+}{\sqrt{2}},
\qquad
x^{(-)} := \frac{e_0+a_-}{\sqrt{2}}.
\]
Each lifted action has norm $1$, so the finite action set
\[
\cA_t := \{x^{(0)},x^{(+)},x^{(-)}\}
\qquad \forall t
\]
fits the main setup with $K=3$.

Now define the common offline parameter and the three online parameters by
\[
\tilde\theta^\dagger
:=
\frac{1}{\sqrt{2}}e_0 + \sqrt{2}\rho_0 e_1,
\]
\[
\tilde\theta_+
:=
\frac{1}{\sqrt{2}}e_0 + \sqrt{2}\bigl(\rho_0 e_1 + \bar{\rho} e_2\bigr),
\qquad
\tilde\theta_-
:=
\frac{1}{\sqrt{2}}e_0 + \sqrt{2}\bigl(\rho_0 e_1 - \bar{\rho} e_2\bigr),
\]
\[
\tilde\theta_{\mathrm{good}}
:=
\frac{1}{\sqrt{2}}e_0 + \sqrt{2}(\rho_0+\bar{\rho})e_1.
\]
For notational continuity with the statement, write these three online parameters as
$\theta_+,\theta_-,\theta_{\mathrm{good}}$ and the common offline parameter as $\theta^\dagger$.
Take any deterministic offline covariates $\{z_i\}$ with $\|z_i\|_2\le 1$ and
$z_i^\top \theta^\dagger \in [0,1]$, and let the offline rewards be Bernoulli with means
$z_i^\top \theta^\dagger$. Online rewards are also Bernoulli, with mean $x^\top \theta$ when action
$x\in\cA_t$ is played under parameter $\theta$.

All displayed online means lie in $[1/2,13/16]$: the smallest is
$1/2 + (\rho_0^2-\bar{\rho}^2)/\sqrt{\rho_0^2+\bar{\rho}^2} \ge 1/2$, and the largest is
$1/2+\rho_0+\bar{\rho} \le 13/16$ because $\rho_0\le 1/4$ and $0<\rho\le \rho_0/4$.
Hence rewards are in $[0,1]$, and the centered Bernoulli noise is conditionally sub-Gaussian.

The three instances all use the same offline parameter $\theta^\dagger$ and the same deterministic
offline covariates. Therefore the law of $D_{\mathrm{off}}$ is identical across all three instances.
Moreover,
\[
\norm{\theta_+ - \theta^\dagger}_2
=
\norm{\theta_- - \theta^\dagger}_2
=
\norm{\theta_{\mathrm{good}} - \theta^\dagger}_2
=
\rho,
\]
so the same isotropic certificate is valid throughout.

For the hard family, let $P_+$ and $P_-$ denote the laws of the full online interaction under
$\theta_+$ and $\theta_-$, respectively. Let $v:=e_2$, and define the event
\[
E:=\left\{\sum_{t=1}^T \mathbf{1}\{\ip{v}{x_t}\ge 0\}\ge \frac{T}{2}\right\}.
\]
Under $\theta_-$, the unique optimal action in $\cA_t$ is $x^{(-)}$, whose mean
reward equals
\[
(x^{(-)})^\top \theta_- = \frac{1}{2} + \sqrt{\rho_0^2+\bar{\rho}^2}.
\]
For any chosen action $x_t\in\cA_t$, write
\[
x_t = \frac{e_0+a_t}{\sqrt{2}}
\qquad\text{with}\qquad
a_t\in\{a_0,a_+,a_-\}.
\]
Any action with $\ip{v}{x_t}\ge 0$ is either $x^{(0)}$ or $x^{(+)}$, and each satisfies
\[
x_t^\top \theta_-
=
\frac{1}{2} + \rho_0 \ip{e_1}{a_t} - \bar{\rho}\ip{v}{a_t}
\le
\frac{1}{2} + \rho_0.
\]
Hence every round in $E$ incurs regret at least
\[
\sqrt{\rho_0^2+\bar{\rho}^2} - \rho_0
\ge
\frac{\bar{\rho}^2}{4\rho_0}
=
\frac{\rho^2}{8\rho_0},
\]
where the last inequality uses $\bar{\rho} \le \rho_0/4$. Therefore,
\[
R_T(\theta_-)\ge \frac{\rho^2 T}{16\rho_0}
\qquad \text{on } E.
\]
By symmetry,
\[
R_T(\theta_+)\ge \frac{\rho^2 T}{16\rho_0}
\qquad \text{on } E^c.
\]

The offline KL divergence between the two hard instances is zero because the offline law is the same.
For the online interaction, if the chosen action at round $t$ has Bernoulli means
$p_t:=x_t^\top\theta_+$ and $q_t:=x_t^\top\theta_-$, then
\[
\mathrm{kl}(p_t,q_t)
\le
\frac{(p_t-q_t)^2}{q_t(1-q_t)}
\le
\frac{256}{39}(p_t-q_t)^2,
\]
because $q_t\in[1/2,13/16]$. Moreover, $p_t-q_t=0$ for $x_t=x^{(0)}$, while for
$x_t\in\{x^{(+)},x^{(-)}\}$,
\[
|p_t-q_t|
=
\left|x_t^\top(\theta_+-\theta_-)\right|
=
\frac{2\bar{\rho}^2}{\sqrt{\rho_0^2+\bar{\rho}^2}}
\le
\frac{2\bar{\rho}^2}{\rho_0}.
\]
Hence every round contributes at most
\[
\mathrm{kl}(p_t,q_t)
\le
\frac{1024}{39}\frac{\bar{\rho}^4}{\rho_0^2}
\le
\frac{64}{39}\bar{\rho}^2
=
\frac{32}{39}\rho^2,
\]
where the second inequality again uses $\bar{\rho}\le \rho_0/4$. By the chain rule,
\[
\mathrm{KL}(P_+\,\|\,P_-)\le \frac{32}{39}\rho^2T.
\]
Thus $\mathrm{KL}(P_+\,\|\,P_-)\le 1/8$ when $c_0$ is chosen small enough. Bretagnolle--Huber then
gives
\[
P_+(E^c)+P_-(E)\ge \frac{1}{2}e^{-1/8}.
\]
Combining the last three displays yields
\[
\max\{\E_+[R_T],\, \E_-[R_T]\}
\ge
\frac{e^{-1/8}}{64}\frac{\rho^2 T}{\rho_0}.
\]
This proves part (i) after absorbing constants into $c_1$.

For the good instance, the action $x^{(0)}$ has mean
\[
(x^{(0)})^\top \theta_{\mathrm{good}}
=
\frac{1}{2}+\rho_0+\bar{\rho},
\]
whereas
\[
(x^{(\pm)})^\top \theta_{\mathrm{good}}
=
\frac{1}{2}
+
\frac{\rho_0(\rho_0+\bar{\rho})}{\sqrt{\rho_0^2+\bar{\rho}^2}}
<
\frac{1}{2}+\rho_0+\bar{\rho}.
\]
Thus $x^{(0)}$ is optimal at every round, and the deterministic policy that always plays $x^{(0)}$
has zero regret, proving part (ii).

For the final claim, $D_{\mathrm{off}}$ has the same law across the good and hard instances, so any
measurable summary $S=\Phi(D_{\mathrm{off}})$ also has the same distribution. Hence no offline-only
summary can identify from the offline sample alone whether the learner is in the easy instance or in
the hard family above, even though their online regret behavior is different.
\end{proof}

\section{Notation}
\label{app:notation}

Table~\ref{tab:notation} collects recurrent symbols. The layerwise procedure is stated as
Algorithm~\ref{alg:ellipsoidal-minucb} in the main text.

\begin{table}[h]
\centering
\caption{Main notation.}
\label{tab:notation}
\small
\setlength{\tabcolsep}{5pt}
\begin{tabular}{@{}p{0.26\linewidth}p{0.68\linewidth}@{}}
\toprule
\textbf{Symbol} & \textbf{Meaning} \\
\midrule
$T,K,d$ & Horizon, number of actions per round, feature dimension. \\
$\theta_*$ & Unknown online reward parameter; $\|\theta_*\|_2\le S$. \\
$\theta^\dagger$ & Offline regression parameter in $y_i=z_i^\top\theta^\dagger+\xi_i$. \\
$D_{\mathrm{off}},n_{\mathrm{off}}$ & Offline sample $\{(z_i,y_i)\}$ and its size. \\
$G_{\mathrm{off}},\hat\theta_{\mathrm{off}},\beta_{\mathrm{off}}(\delta)$ & Offline ridge design
$I+\sum_i z_i z_i^\top$, ridge estimator, and offline concentration radius. \\
$(M_{\mathrm{shift}},\rho)$ & Shift certificate: $\|\theta_*-\theta^\dagger\|_{M_{\mathrm{shift}}}\le\rho$. \\
$\cF_{t-1}$ & Filtration generated by past data and current contexts (Section~\ref{sec:setup}). \\
$\ell,L$ & SupLinUCB layer index; $L=\lceil\log_2 T\rceil$. \\
$\cH_{t,\ell}$ & History routed to layer $\ell$ before round $t$. \\
$A_{t,\ell},V_{t,\ell},b_{t,\ell}$ & Layerwise online Gram matrix, $V_{t,\ell}=I+A_{t,\ell}$, and response vector
$b_{t,\ell}$ on layer $\ell$ (Section~\ref{sec:algorithm}). \\
$\hat\theta^{\mathrm{on}}_{t,\ell},\hat\theta^{\mathrm{pool}}_{t,\ell}$ & Online and pooled ridge estimators on layer $\ell$. \\
$\beta^{\mathrm{on}}_{t,\ell},\gamma_{t,\ell}$ & Online SupLin radius and pooled martingale radius. \\
$\psi_{t,\ell}(x)$ & Shift routing term in the pooled radius (Section~\ref{sec:algorithm}). \\
$U^{\mathrm{on}},U^{\mathrm{pool}},U^{\min},L^{\max},w$ & Branch UCB/LCB scores and aggregated width. \\
$\delta_{\mathrm{off}},\delta^{\mathrm{on}}_{t,\ell},\delta^{\mathrm{pool}}_{t,\ell}$ & Confidence budgets in Theorem~\ref{thm:main}. \\
$\widetilde\Lambda_T,\widetilde\Psi_T$ & Offline design log-det sum and path sum of $\psi$ (Theorem~\ref{thm:main}). \\
$A^{\mathrm{fin}}_\ell$ & Final Gram matrix on layer $\ell$ at horizon $T$. \\
$\beta_\star,\delta_{\min}^{\mathrm{pool}}$ & Pooled-radius shorthand in Theorem~\ref{thm:main}. \\
$\Delta_{t,\ell}(x),h_{\mathrm{off}}(x)$ & Directional helpfulness gap and offline summary (Section~\ref{sec:algorithm}). \\
\bottomrule
\end{tabular}
\end{table}

\section{Proof of Proposition~\ref{prop:offline-region}}

We expand the two ingredients that enter the proposition: the offline ridge concentration event and
the support function of the resulting confidence region.

\begin{proof}
Condition on the offline covariates $\{z_i\}_{i=1}^{n_{\mathrm{off}}}$. The imported
self-normalized ridge inequality states that, with probability at least $1-\delta$,
\[
\|\hat\theta_{\mathrm{off}}-\theta^\dagger\|_{G_{\mathrm{off}}}
\le
\beta_{\mathrm{off}}(\delta).
\]
On the same event, the directional certificate gives
\[
\|\theta_*-\theta^\dagger\|_{M_{\mathrm{shift}}}\le \rho.
\]
Write
\[
\theta_*-\hat\theta_{\mathrm{off}}
=
(\theta^\dagger-\hat\theta_{\mathrm{off}})+(\theta_*-\theta^\dagger)
=:u+v.
\]
Then
\[
\|u\|_{G_{\mathrm{off}}}
=
\|\hat\theta_{\mathrm{off}}-\theta^\dagger\|_{G_{\mathrm{off}}}
\le \beta_{\mathrm{off}}(\delta),
\qquad
\|v\|_{M_{\mathrm{shift}}}
=
\|\theta_*-\theta^\dagger\|_{M_{\mathrm{shift}}}
\le \rho.
\]
Hence
\[
\theta_*=\hat\theta_{\mathrm{off}}+u+v
\]
with $u$ and $v$ belonging to the two ellipsoids claimed in the proposition, which proves the region
inclusion.

It remains to compute the support function. Let
\[
\theta=\hat\theta_{\mathrm{off}}+u+v
\]
with $\|u\|_{G_{\mathrm{off}}}\le \beta_{\mathrm{off}}$ and $\|v\|_{M_{\mathrm{shift}}}\le \rho$.
Then
\[
x^\top \theta
=
x^\top \hat\theta_{\mathrm{off}} + x^\top u + x^\top v.
\]
By Cauchy--Schwarz in the $G_{\mathrm{off}}$ metric,
\[
x^\top u
=
(G_{\mathrm{off}}^{-1/2}x)^\top(G_{\mathrm{off}}^{1/2}u)
\le
\|x\|_{G_{\mathrm{off}}^{-1}}\|u\|_{G_{\mathrm{off}}}
\le
\beta_{\mathrm{off}}\|x\|_{G_{\mathrm{off}}^{-1}}.
\]
Likewise,
\[
x^\top v
=
(M_{\mathrm{shift}}^{-1/2}x)^\top(M_{\mathrm{shift}}^{1/2}v)
\le
\|x\|_{M_{\mathrm{shift}}^{-1}}\|v\|_{M_{\mathrm{shift}}}
\le
\rho\|x\|_{M_{\mathrm{shift}}^{-1}}.
\]
This yields the upper bound
\[
x^\top \theta
\le
x^\top\hat\theta_{\mathrm{off}}
+\beta_{\mathrm{off}}\|x\|_{G_{\mathrm{off}}^{-1}}
+\rho\|x\|_{M_{\mathrm{shift}}^{-1}}.
\]
Equality is achieved by choosing $u$ and $v$ aligned with the dual directions
$G_{\mathrm{off}}^{-1}x$ and $M_{\mathrm{shift}}^{-1}x$, respectively. Therefore the upper bound is
the exact support function.
\end{proof}

\begin{lemma}[Support function of the offline region]
\label{lem:support}
Under the event of Proposition~\ref{prop:offline-region}, every $x\in\R^d$ satisfies
\[
\sup_{\theta \in \cC_{\mathrm{off}}} x^{\top}\theta
=
x^{\top}\hat\theta_{\mathrm{off}}
+ \beta_{\mathrm{off}}\|x\|_{G_{\mathrm{off}}^{-1}}
+ \rho\|x\|_{M_{\mathrm{shift}}^{-1}}.
\]
\end{lemma}

\begin{proof}
This is exactly the support-function computation established in the proof of
Proposition~\ref{prop:offline-region}.
\end{proof}

\section{Imported Self-Normalized Tools}
\label{app:self-normalized}

Nothing in this section is new. We record the standard self-normalized derivation only because it is
used twice in our paper: once for the offline ridge estimator and once for masked martingale sums
that define the layerwise online and pooled histories. We specialize to ridge level $1$, matching
Section~\ref{sec:setup}.
Replacing $I$ by $\lambda I$ recovers the usual $\sqrt{\lambda}$ and $\log(1+T/\lambda)$ dependence.

\begin{lemma}[Self-normalized martingale term]
\label{lem:self-normalized-noise}
Let $(\cF_s)_{s=0}^n$ be a filtration. Suppose $\phi_s \in \R^d$ is $\cF_{s-1}$-measurable with
$\|\phi_s\|_2\le 1$, and $\eta_s$ is conditionally $\sigma$-sub-Gaussian given $\cF_{s-1}$. Define
\[
Z_t:=\sum_{s=1}^t \phi_s \eta_s,
\qquad
V_t:=I+\sum_{s=1}^t \phi_s\phi_s^\top.
\]
Then, for every $\delta\in(0,1)$,
\[
\Prb\!\left(
\|Z_n\|_{V_n^{-1}}
\le
\sigma\sqrt{2\log\frac{\det(V_n)^{1/2}}{\delta}}
\right)
\ge 1-\delta.
\]
\end{lemma}

\begin{proof}
Fix $\nu\in\R^d$ and define
\[
M_t(\nu)
:=
\exp\left(
\sigma^{-1}\ip{\nu}{Z_t}
-\frac12 \nu^\top(V_t-I)\nu
\right).
\]
Since $\phi_t$ is $\cF_{t-1}$-measurable and $\eta_t$ is conditionally $\sigma$-sub-Gaussian,
\[
\E\!\left[
\exp\left(\sigma^{-1}\eta_t\ip{\nu}{\phi_t}\right)\middle|\cF_{t-1}
\right]
\le
\exp\left(\frac12\ip{\nu}{\phi_t}^2\right).
\]
Therefore
\[
\E\!\left[\frac{M_t(\nu)}{M_{t-1}(\nu)}\middle|\cF_{t-1}\right]\le 1,
\]
so $(M_t(\nu))_{t=0}^n$ is a nonnegative supermartingale and $\E[M_n(\nu)]\le 1$.

Now mix over $\nu$ with the Gaussian density
\[
f(\nu)
:=
\frac{1}{(2\pi)^{d/2}}
\exp\left(-\frac12\nu^\top\nu\right),
\]
and define
\[
\widetilde M_n:=\int_{\R^d} M_n(\nu)f(\nu)\,d\nu.
\]
By Fubini,
\[
\E[\widetilde M_n]
=
\int_{\R^d} \E[M_n(\nu)]f(\nu)\,d\nu
\le
\int_{\R^d} f(\nu)\,d\nu
=1.
\]
Combining the definitions of $M_n(\nu)$ and $f(\nu)$ gives
\[
\widetilde M_n
=
\frac{1}{(2\pi)^{d/2}}
\int_{\R^d}
\exp\left(
\sigma^{-1}\ip{\nu}{Z_n}-\frac12\nu^\top V_n\nu
\right)d\nu.
\]
Completing the square,
\[
\sigma^{-1}\ip{\nu}{Z_n}-\frac12\nu^\top V_n\nu
=
-\frac12\left\|\nu-\sigma^{-1}V_n^{-1}Z_n\right\|_{V_n}^2
+ \frac{1}{2\sigma^2}\|Z_n\|_{V_n^{-1}}^2.
\]
Hence
\[
\widetilde M_n
=
\frac{1}{(2\pi)^{d/2}}
\exp\left(\frac{1}{2\sigma^2}\|Z_n\|_{V_n^{-1}}^2\right)
\int_{\R^d}
\exp\left(
-\frac12\left\|\nu-\sigma^{-1}V_n^{-1}Z_n\right\|_{V_n}^2
\right)d\nu.
\]
The remaining Gaussian integral equals $(2\pi)^{d/2}\det(V_n)^{-1/2}$, so
\[
\widetilde M_n
=
\frac{1}{\det(V_n)^{1/2}}
\exp\left(\frac{1}{2\sigma^2}\|Z_n\|_{V_n^{-1}}^2\right).
\]
Markov's inequality and $\E[\widetilde M_n]\le 1$ imply
\[
\Prb\!\left(\widetilde M_n\ge \delta^{-1}\right)\le \delta.
\]
Rearranging the event $\widetilde M_n\le \delta^{-1}$ yields the claim.
\end{proof}

\begin{proposition}[Ridge confidence ellipsoid]
\label{prop:derive-self-normalized}
Under the assumptions of Lemma~\ref{lem:self-normalized-noise}, let
\[
Y_s=\phi_s^\top \theta + \eta_s,
\qquad
\hat\theta_n:=V_n^{-1}\sum_{s=1}^n \phi_sY_s,
\qquad
\|\theta\|_2\le S.
\]
Then, with probability at least $1-\delta$,
\[
\|\hat\theta_n-\theta\|_{V_n}
\le
\sigma\sqrt{2\log\frac{\det(V_n)^{1/2}}{\delta}}
+S.
\]
\end{proposition}

\begin{proof}
Using $Y_s=\phi_s^\top\theta+\eta_s$,
\[
V_n\hat\theta_n
=
\sum_{s=1}^n \phi_sY_s
=
\sum_{s=1}^n \phi_s\phi_s^\top\theta+\sum_{s=1}^n \phi_s\eta_s
=
(V_n-I)\theta+Z_n.
\]
Therefore
\[
V_n(\hat\theta_n-\theta)=Z_n-\theta.
\]
Taking the $V_n^{-1}$ norm and applying the triangle inequality,
\[
\|\hat\theta_n-\theta\|_{V_n}
=
\|Z_n-\theta\|_{V_n^{-1}}
\le
\|Z_n\|_{V_n^{-1}}+\|\theta\|_{V_n^{-1}}.
\]
Lemma~\ref{lem:self-normalized-noise} controls the first term. Since $V_n\succeq I$, we have
$V_n^{-1}\preceq I$, hence
\[
\|\theta\|_{V_n^{-1}}
\le
\|\theta\|_2
\le
S.
\]
Combining the two bounds proves the result.
\end{proof}

\begin{lemma}[Predictable masks]
\label{lem:subsequence-self-normalized}
Let $(\cF_s)_{s=0}^T$ be a filtration. Suppose $\phi_s$ is $\cF_{s-1}$-measurable and $\eta_s$ is
conditionally $\sigma$-sub-Gaussian given $\cF_{s-1}$. Let $m_s\in[0,1]$ be
$\cF_{s-1}$-measurable. Define
\[
\widetilde Z_t := \sum_{s=1}^t m_s \phi_s\eta_s,
\qquad
\widetilde V_t := I+\sum_{s=1}^t m_s^2 \phi_s\phi_s^\top.
\]
Then, with probability at least $1-\delta$,
\[
\|\widetilde Z_T\|_{\widetilde V_T^{-1}}
\le
\sigma\sqrt{2\log\frac{\det(\widetilde V_T)^{1/2}}{\delta}}.
\]
\end{lemma}

\begin{proof}
Set $\widetilde\phi_s:=m_s\phi_s$. Since $m_s$ and $\phi_s$ are both $\cF_{s-1}$-measurable,
$\widetilde\phi_s$ is predictable. Moreover $\|\widetilde\phi_s\|_2\le \|\phi_s\|_2\le 1$ because
$m_s\in[0,1]$. Applying Lemma~\ref{lem:self-normalized-noise} to the predictable pair
$(\widetilde\phi_s,\eta_s)$ yields the claim.
\end{proof}

\section{Confidence Events and Elimination Lemmas}

This section supplies the entire logical chain behind the main theorem: simultaneous confidence,
combined UCB and LCB validity, survival of the optimal arm, and the stopping-layer regret bound.

For each round let
\[
a_t^\star \in \argmax_{a\in[K]} x_{t,a}^\top\theta_*,
\qquad
\Delta_t(a):=x_{t,a_t^\star}^\top\theta_* - x_{t,a}^\top\theta_*.
\]
Let $\cA_{t,\ell}$ denote the set of arms surviving through layer $\ell$ on round $t$, and let
$\ell_t$ be the stopping layer on round $t$. Define the widths
\[
w_{t,\ell}(a)
:=
U_{t,\ell}^{\min}(a)-L_{t,\ell}^{\max}(a),
\qquad
w_{t,\ell}^{\mathrm{on}}(a)
:=
U_{t,\ell}^{\mathrm{on}}(a)-L_{t,\ell}^{\mathrm{on}}(a),
\]
and similarly
$w_{t,\ell}^{\mathrm{pool}}(a):=U_{t,\ell}^{\mathrm{pool}}(a)-L_{t,\ell}^{\mathrm{pool}}(a)$.

\begin{lemma}[Width comparison]
\label{lem:width-comparison}
For every round, layer, and action,
\[
w_{t,\ell}(a)\le \min\{w_{t,\ell}^{\mathrm{on}}(a),w_{t,\ell}^{\mathrm{pool}}(a)\}
\le w_{t,\ell}^{\mathrm{on}}(a),
\]
and
\[
w_{t,\ell}(a)\le w_{t,\ell}^{\mathrm{pool}}(a)
=2\,\mathrm{rad}^{\mathrm{pool}}_{t,\ell}(x_{t,a}).
\]
\end{lemma}

\begin{proof}
By definition,
\[
w_{t,\ell}(a)
=
\min\{U_{t,\ell}^{\mathrm{on}}(a),U_{t,\ell}^{\mathrm{pool}}(a)\}
-\max\{L_{t,\ell}^{\mathrm{on}}(a),L_{t,\ell}^{\mathrm{pool}}(a)\}.
\]
For any numbers $u_1,u_2,\ell_1,\ell_2$,
\[
\min\{u_1,u_2\}-\max\{\ell_1,\ell_2\}
\le
\min\{u_1-\ell_1,u_2-\ell_2\}.
\]
Applying this with the online and pooled endpoints proves the first display. The second follows from
the explicit form of the pooled UCB--LCB pair.
\end{proof}

Choose confidence levels so that
\[
\sum_{t=1}^T\sum_{\ell=0}^{\lceil \log_2 T\rceil}\delta_{t,\ell}^{\mathrm{on}}
\le \delta_{\mathrm{on}},
\qquad
\delta_{\mathrm{off}}+\delta_{\mathrm{on}}
+\sum_{t=1}^T\sum_{\ell=0}^{\lceil \log_2 T\rceil}\delta_{t,\ell}^{\mathrm{pool}}
\le T^{-2},
\]
abbreviate $\beta_{\mathrm{off}}:=\beta_{\mathrm{off}}(\delta_{\mathrm{off}})$, set
\[
L_T:=\log\!\Bigl(\frac{2KT\log T}{\delta_{\mathrm{on}}}\Bigr).
\]
Also define
\[
\cE_{t,\ell}^{\mathrm{on}}
:=
\left\{
\|b_{t,\ell}-A_{t,\ell}\theta_*\|_{V_{t,\ell}^{-1}}
\le
\beta^{\mathrm{on}}_{t,\ell}-S
\right\}.
\]
Define the events
\[
\cE_{\mathrm{off}}
:=
\left\{\|\hat\theta_{\mathrm{off}}-\theta^\dagger\|_{G_{\mathrm{off}}}\le \beta_{\mathrm{off}}\right\},
\]
\[
\cE_{t,\ell}^{\mathrm{pool}}
:=
\left\{\|b_{t,\ell}-A_{t,\ell}\theta_*\|_{V_{t,\ell}^{-1}}\le \gamma_{t,\ell}\right\},
\]
\[
\cE_{\mathrm{on}}
:=
\bigcap_{t=1}^T\bigcap_{\ell=0}^{\lceil \log_2 T\rceil}\cE_{t,\ell}^{\mathrm{on}},
\]
and finally set
\[
\cE
:=
\cE_{\mathrm{on}}
\cap
\cE_{\mathrm{off}}
\cap
\bigcap_{t=1}^T\bigcap_{\ell=0}^{\lceil \log_2 T\rceil}\cE_{t,\ell}^{\mathrm{pool}}.
\]

\begin{lemma}[Simultaneous confidence event]
\label{lem:joint-event}
We have $\Prb(\cE)\ge 1-T^{-2}$.
\end{lemma}

\begin{proof}
By the offline ridge bound,
\[
\Prb(\cE_{\mathrm{off}})\ge 1-\delta_{\mathrm{off}}.
\]
Fix $(t,\ell)$ and define the predictable mask
\[
m_s^{(t,\ell)}:=\mathbf{1}\{s<t,\ s\in\cH_{t,\ell}\},
\qquad s=1,\dots,T.
\]
Because the action set at round $s$ is revealed before the layer assignment and action choice, the
event $\{s\in\cH_{t,\ell}\}$ is determined by information available at time $s-1$ together with the
current contexts; hence $m_s^{(t,\ell)}$ is $\cF_{s-1}$-measurable. Therefore
\[
b_{t,\ell}-A_{t,\ell}\theta_*
=
\sum_{s=1}^{T} m_s^{(t,\ell)}x_{s,a_s}\eta_s,
\qquad
\eta_s:=r_s-x_{s,a_s}^\top\theta_*,
\]
and
\[
V_{t,\ell}
=
I+\sum_{s=1}^{T} m_s^{(t,\ell)}x_{s,a_s}x_{s,a_s}^\top.
\]
Applying Lemma~\ref{lem:subsequence-self-normalized} with
$\phi_s=x_{s,a_s}$ and mask $m_s^{(t,\ell)}$ gives
\[
\|b_{t,\ell}-A_{t,\ell}\theta_*\|_{V_{t,\ell}^{-1}}
\le
\sigma\sqrt{2\log\frac{\det(V_{t,\ell})^{1/2}}{\delta_{t,\ell}^{\mathrm{pool}}}}
\]
with probability at least $1-\delta_{t,\ell}^{\mathrm{pool}}$. Since $\gamma_{t,\ell}$ adds the
nonnegative term $S$, the same event implies $\cE_{t,\ell}^{\mathrm{pool}}$. Thus
\[
\Prb(\cE_{t,\ell}^{\mathrm{pool}})\ge 1-\delta_{t,\ell}^{\mathrm{pool}}.
\]
The same masked bound with confidence level $\delta_{t,\ell}^{\mathrm{on}}$ yields
\[
\Prb(\cE_{t,\ell}^{\mathrm{on}})\ge 1-\delta_{t,\ell}^{\mathrm{on}}.
\]
Applying the union bound over all $(t,\ell)$ and using
$\sum_{t,\ell}\delta_{t,\ell}^{\mathrm{on}}\le \delta_{\mathrm{on}}$ gives
\[
\Prb(\cE_{\mathrm{on}})\ge 1-\delta_{\mathrm{on}}.
\]
Applying the union bound over $\cE_{\mathrm{off}}^c$, $\cE_{\mathrm{on}}^c$, and all pooled events
gives
\[
\Prb(\cE^c)
\le
\delta_{\mathrm{off}}+\delta_{\mathrm{on}}
+\sum_{t,\ell}\delta_{t,\ell}^{\mathrm{pool}}
\le T^{-2}.
\]
\end{proof}

\begin{lemma}[Validity of the pooled branch]
\label{lem:pooled-valid}
Fix a round-layer pair $(t,\ell)$. On the event
$\cE_{\mathrm{off}}\cap \cE_{t,\ell}^{\mathrm{pool}}$, every action $a$ satisfies
\[
\left|
x_{t,a}^\top(\hat\theta_{t,\ell}^{\mathrm{pool}}-\theta_*)
\right|
\le
(\gamma_{t,\ell}+\beta_{\mathrm{off}})
\|x_{t,a}\|_{(A_{t,\ell}+G_{\mathrm{off}})^{-1}}
+ \rho\,\psi_{t,\ell}(x_{t,a}).
\]
\end{lemma}

\begin{proof}
Write $A:=A_{t,\ell}$, $G:=G_{\mathrm{off}}$, and $x:=x_{t,a}$. Expanding the pooled estimator,
\[
\hat\theta_{t,\ell}^{\mathrm{pool}}-\theta_*
=(A+G)^{-1}
\Bigl[
(b_{t,\ell}-A\theta_*)
+G(\hat\theta_{\mathrm{off}}-\theta^\dagger)
+G(\theta^\dagger-\theta_*)
\Bigr].
\]
Therefore
\[
\left|x^\top(\hat\theta_{t,\ell}^{\mathrm{pool}}-\theta_*)\right|
\le |T_1|+|T_2|+|T_3|,
\]
where
\[
T_1:=x^\top(A+G)^{-1}(b_{t,\ell}-A\theta_*),
\quad
T_2:=x^\top(A+G)^{-1}G(\hat\theta_{\mathrm{off}}-\theta^\dagger),
\]
\[
T_3:=x^\top(A+G)^{-1}G(\theta^\dagger-\theta_*).
\]
For $T_1$, set $u:=(A+G)^{-1}x$. Then
\[
|T_1|
=
|u^\top(b_{t,\ell}-A\theta_*)|
\le
\|u\|_{V_{t,\ell}}\|b_{t,\ell}-A\theta_*\|_{V_{t,\ell}^{-1}}.
\]
Since $V_{t,\ell}=I + A\preceq A+G$, we have
\[
\|u\|_{V_{t,\ell}}^2
=
x^\top(A+G)^{-1}V_{t,\ell}(A+G)^{-1}x
\le
x^\top(A+G)^{-1}x.
\]
Using $\cE_{t,\ell}^{\mathrm{pool}}$ yields
\[
|T_1|\le \gamma_{t,\ell}\|x\|_{(A+G)^{-1}}.
\]
For $T_2$, write
\[
|T_2|
=
\left|
\bigl(G^{1/2}(A+G)^{-1}x\bigr)^\top
\bigl(G^{1/2}(\hat\theta_{\mathrm{off}}-\theta^\dagger)\bigr)
\right|
\]
and apply Cauchy--Schwarz:
\[
|T_2|
\le
\|x\|_{(A+G)^{-1}G(A+G)^{-1}}
\|\hat\theta_{\mathrm{off}}-\theta^\dagger\|_G.
\]
Because $G\preceq A+G$,
\[
(A+G)^{-1}G(A+G)^{-1}\preceq (A+G)^{-1},
\]
so on $\cE_{\mathrm{off}}$,
\[
|T_2|\le \beta_{\mathrm{off}}\|x\|_{(A+G)^{-1}}.
\]
For $T_3$, let $w:=G(A+G)^{-1}x$. Then
\[
|T_3|=|w^\top(\theta^\dagger-\theta_*)|
\le
\rho\|w\|_{M_{\mathrm{shift}}^{-1}}
=
\rho\,\psi_{t,\ell}(x)
\]
by the certificate. Summing the three bounds proves the claim.
\end{proof}

\begin{lemma}[Combined UCB and LCB validity]
\label{lem:combined-valid}
On $\cE$, every round-layer-action triple satisfies
\[
x_{t,a}^\top\theta_*
\in
[L_{t,\ell}^{\max}(a),U_{t,\ell}^{\min}(a)].
\]
\end{lemma}

\begin{proof}
On $\cE$, the pooled UCB--LCB pair is valid by Lemma~\ref{lem:pooled-valid}. For the online branch,
\[
\hat\theta^{\mathrm{on}}_{t,\ell}-\theta_*
=
V_{t,\ell}^{-1}(b_{t,\ell}-A_{t,\ell}\theta_*)-V_{t,\ell}^{-1}\theta_*.
\]
Thus
\[
\|\hat\theta^{\mathrm{on}}_{t,\ell}-\theta_*\|_{V_{t,\ell}}
\le
\|b_{t,\ell}-A_{t,\ell}\theta_*\|_{V_{t,\ell}^{-1}}
+ \|\theta_*\|_{V_{t,\ell}^{-1}}
\le
(\beta^{\mathrm{on}}_{t,\ell}-S)+S
=
\beta^{\mathrm{on}}_{t,\ell}
\]
on $\cE_{t,\ell}^{\mathrm{on}}$, since $V_{t,\ell}\succeq I$ and $\|\theta_*\|_2\le S$. Therefore
$|x_{t,a}^\top(\hat\theta_{t,\ell}^{\mathrm{on}}-\theta_*)|
\le \beta^{\mathrm{on}}_{t,\ell}\|x_{t,a}\|_{V_{t,\ell}^{-1}}$ on $\cE$, so the online pair is
also valid. Therefore
\[
x_{t,a}^\top\theta_*
\le
\min\{U_{t,\ell}^{\mathrm{on}}(a),U_{t,\ell}^{\mathrm{pool}}(a)\}
=
U_{t,\ell}^{\min}(a)
\]
and similarly
\[
x_{t,a}^\top\theta_*
\ge
\max\{L_{t,\ell}^{\mathrm{on}}(a),L_{t,\ell}^{\mathrm{pool}}(a)\}
=
L_{t,\ell}^{\max}(a).
\]
\end{proof}

\begin{lemma}[Optimal action survives elimination]
\label{lem:optimal-survives}
On $\cE$, for every round $t$ and layer $\ell$,
\[
a_t^\star \in \cA_{t,\ell}.
\]
\end{lemma}

\begin{proof}
The base case $\ell=0$ is immediate since $\cA_{t,0}=[K]$. Suppose
$a_t^\star\in \cA_{t,\ell}$ and the algorithm descends to layer $\ell+1$. By definition,
\[
m_{t,\ell}:=\max_{a\in \cA_{t,\ell}} L_{t,\ell}^{\max}(a).
\]
Lemma~\ref{lem:combined-valid} implies
\[
L_{t,\ell}^{\max}(a)\le x_{t,a}^\top\theta_* \le x_{t,a_t^\star}^\top\theta_*
\le U_{t,\ell}^{\min}(a_t^\star)
\qquad
\text{for all } a\in \cA_{t,\ell}.
\]
Therefore
\[
U_{t,\ell}^{\min}(a_t^\star)\ge m_{t,\ell},
\]
so the optimal action is not eliminated and remains in $\cA_{t,\ell+1}$.
\end{proof}

\begin{lemma}[Survivor quality after a narrow layer]
\label{lem:survivor-quality}
On $\cE$, fix $t$ and $\ell<\lceil\log_2 T\rceil$. If every arm in $\cA_{t,\ell}$ satisfies
$w_{t,\ell}(a)\le 2^{-\ell}$ and the algorithm descends to layer $\ell+1$, then every
$a\in \cA_{t,\ell+1}$ obeys
\[
\Delta_t(a)\le 2^{1-\ell}.
\]
\end{lemma}

\begin{proof}
Take $a\in \cA_{t,\ell+1}$. By the elimination rule,
\[
U_{t,\ell}^{\min}(a)\ge m_{t,\ell}\ge L_{t,\ell}^{\max}(a_t^\star).
\]
Hence
\begin{align*}
\Delta_t(a)
&=
x_{t,a_t^\star}^\top\theta_* - x_{t,a}^\top\theta_* \\
&=
\bigl(x_{t,a_t^\star}^\top\theta_* - L_{t,\ell}^{\max}(a_t^\star)\bigr)
+\bigl(L_{t,\ell}^{\max}(a_t^\star)-U_{t,\ell}^{\min}(a)\bigr)
+\bigl(U_{t,\ell}^{\min}(a)-x_{t,a}^\top\theta_*\bigr).
\end{align*}
The middle term is nonpositive, and the first and third terms are each at most $2^{-\ell}$ by
Lemma~\ref{lem:combined-valid} and the width assumption. Thus
\[
\Delta_t(a)\le 2^{-\ell}+2^{-\ell}=2^{1-\ell}.
\]
\end{proof}

\begin{corollary}[Layer invariant]
\label{cor:layer-invariant}
On $\cE$, every round $t$ and every layer $\ell\ge 1$ satisfy
\[
\Delta_t(a)\le 2^{2-\ell}
\qquad
\text{for all } a\in \cA_{t,\ell}.
\]
\end{corollary}

\begin{proof}
On $\cE$, apply Lemma~\ref{lem:survivor-quality} at layer $\ell-1$.
\end{proof}

\begin{lemma}[Stopping-layer regret bound]
\label{lem:stopping-regret}
On $\cE$, every round $t$ satisfies
\[
\Delta_t(a_t)
\le
4\min\{1,w_{t,\ell_t}(a_t)\}
\le
8\min\{1,\mathrm{rad}_{t,\ell_t}^{\mathrm{pool}}(x_{t,a_t})\}.
\]
\end{lemma}

\begin{proof}
We consider the stopping layer $\ell_t$.

\paragraph{Case 1: $\ell_t=\lceil\log_2 T\rceil$.}
The played arm maximizes $U_{t,\ell_t}^{\min}$ over $\cA_{t,\ell_t}$, and
$a_t^\star\in \cA_{t,\ell_t}$ by Lemma~\ref{lem:optimal-survives}. Therefore
\[
U_{t,\ell_t}^{\min}(a_t)\ge U_{t,\ell_t}^{\min}(a_t^\star)\ge x_{t,a_t^\star}^\top\theta_*.
\]
Using Lemma~\ref{lem:combined-valid},
\[
\Delta_t(a_t)
\le
U_{t,\ell_t}^{\min}(a_t)-L_{t,\ell_t}^{\max}(a_t)
=
w_{t,\ell_t}(a_t).
\]
Also, rewards lie in $[0,1]$, so $\Delta_t(a_t)\le 1$. Hence
\[
\Delta_t(a_t)
\le
\min\{1,w_{t,\ell_t}(a_t)\}
\le
4\min\{1,w_{t,\ell_t}(a_t)\}.
\]

\paragraph{Case 2: $\ell_t<\lceil\log_2 T\rceil$.}
If $\ell_t=0$, then $\Delta_t(a_t)\le 1$ because rewards are bounded in $[0,1]$, and
$1\le 4\min\{1,w_{t,0}(a_t)\}$ since the algorithm stops only when $w_{t,0}(a_t)>1$ or the terminal
layer is reached.

If $\ell_t\ge 1$, Corollary~\ref{cor:layer-invariant} gives
\[
\Delta_t(a_t)\le 2^{2-\ell_t}.
\]
But the stopping rule at a nonterminal layer implies $w_{t,\ell_t}(a_t)>2^{-\ell_t}$, so
\[
4\,w_{t,\ell_t}(a_t)> 4\cdot 2^{-\ell_t}=2^{2-\ell_t}.
\]
Hence $\Delta_t(a_t)\le 4\,w_{t,\ell_t}(a_t)$.

Finally, Lemma~\ref{lem:width-comparison} implies
\[
w_{t,\ell_t}(a_t)\le 2\,\mathrm{rad}_{t,\ell_t}^{\mathrm{pool}}(x_{t,a_t}),
\]
so
\[
4\min\{1,w_{t,\ell_t}(a_t)\}
\le
4\min\{1,2\,\mathrm{rad}_{t,\ell_t}^{\mathrm{pool}}(x_{t,a_t})\}
\le
8\min\{1,\mathrm{rad}_{t,\ell_t}^{\mathrm{pool}}(x_{t,a_t})\},
\]
which yields the second bound.
\end{proof}

\begin{corollary}[Mixed-branch master bound]
\label{cor:mixed-branch-master}
On $\cE$, every round $t$ satisfies
\[
\Delta_t(a_t)
\le
8\min\left\{
1,\,
\mathrm{rad}^{\mathrm{on}}_{t,\ell_t}(x_{t,a_t}),\,
\mathrm{rad}^{\mathrm{pool}}_{t,\ell_t}(x_{t,a_t})
\right\}.
\]
Consequently,
\[
R_T
\le
8\sum_{t=1}^T
\min\left\{
1,\,
\mathrm{rad}^{\mathrm{on}}_{t,\ell_t}(x_{t,a_t}),\,
\mathrm{rad}^{\mathrm{pool}}_{t,\ell_t}(x_{t,a_t})
\right\}.
\]
\end{corollary}

\begin{proof}
By Lemma~\ref{lem:stopping-regret},
\[
\Delta_t(a_t)\le 4\min\{1,w_{t,\ell_t}(a_t)\}.
\]
Lemma~\ref{lem:width-comparison} and the explicit online and pooled widths give
\[
w_{t,\ell_t}(a_t)
\le
\min\{w_{t,\ell_t}^{\mathrm{on}}(a_t),w_{t,\ell_t}^{\mathrm{pool}}(a_t)\}
=
2\min\!\left\{
\mathrm{rad}^{\mathrm{on}}_{t,\ell_t}(x_{t,a_t}),
\mathrm{rad}^{\mathrm{pool}}_{t,\ell_t}(x_{t,a_t})
\right\}.
\]
Therefore, if
\[
m_t
:=
\min\!\left\{
\mathrm{rad}^{\mathrm{on}}_{t,\ell_t}(x_{t,a_t}),
\mathrm{rad}^{\mathrm{pool}}_{t,\ell_t}(x_{t,a_t})
\right\},
\]
then
\[
\Delta_t(a_t)
\le
4\min\{1,2m_t\}
\le
8\min\{1,m_t\}
=
8\min\!\left\{
1,\,
\mathrm{rad}^{\mathrm{on}}_{t,\ell_t}(x_{t,a_t}),\,
\mathrm{rad}^{\mathrm{pool}}_{t,\ell_t}(x_{t,a_t})
\right\}.
\]
This proves the first display, and summing over $t$ yields the second.
\end{proof}

\section{Roadmap for the Online Fallback}
\label{app:suplin-roadmap}

The online branch follows the classical SupLinUCB logic. We spell out the two standard ingredients
needed to transfer the fallback bound to our combined UCB/LCB wrapper.

\begin{lemma}[Online width trigger]
\label{lem:online-trigger}
If round $t$ stops at a nonterminal layer $\ell_t$, then
\[
w_{t,\ell_t}^{\mathrm{on}}(a_t)>2^{-\ell_t}.
\]
\end{lemma}

\begin{proof}
The stopping rule gives $w_{t,\ell_t}(a_t)>2^{-\ell_t}$, and
$w_{t,\ell_t}(a_t)\le w_{t,\ell_t}^{\mathrm{on}}(a_t)$ by Lemma~\ref{lem:width-comparison}.
\end{proof}

\begin{lemma}[Layerwise online potential]
\label{lem:online-potential}
Let
\[
Q_\ell:=\{t\in[T]:\ell_t=\ell\}
\]
and
\[
V_{\ell}^{\mathrm{fin}}
:=
I+\sum_{t\in Q_\ell} x_{t,a_t}x_{t,a_t}^\top.
\]
Then
\[
\sum_{t\in Q_\ell}\min\left\{1,\|x_{t,a_t}\|_{V_{t,\ell}^{-1}}^2\right\}
\le
2\log\frac{\det(V_{\ell}^{\mathrm{fin}})}{\det(I)}
\le
2d\log(1+T).
\]
\end{lemma}

\begin{proof}
Enumerate $Q_\ell$ as $t_1<\cdots<t_{|Q_\ell|}$ and define
\[
W_{\ell,0}:=I,
\qquad
W_{\ell,j}:=I+\sum_{i=1}^j x_{t_i,a_{t_i}}x_{t_i,a_{t_i}}^\top.
\]
Then $W_{\ell,j-1}=V_{t_j,\ell}$. By the matrix-determinant lemma,
\[
\det(W_{\ell,j})
=
\det(W_{\ell,j-1})\left(1+\|x_{t_j,a_{t_j}}\|_{W_{\ell,j-1}^{-1}}^2\right).
\]
Summing logarithms gives
\[
\log\frac{\det(V_{\ell}^{\mathrm{fin}})}{\det(I)}
=
\sum_{j=1}^{|Q_\ell|}
\log\left(1+\|x_{t_j,a_{t_j}}\|_{W_{\ell,j-1}^{-1}}^2\right).
\]
Using $\log(1+u)\ge \frac12\min\{u,1\}$ proves the first inequality. The second follows from
AM--GM:
\[
\det(V_{\ell}^{\mathrm{fin}})
\le
\left(1+\frac{T}{d}\right)^d.
\]
\end{proof}

\begin{proposition}[Classical online fallback]
\label{prop:online-fallback}
On $\cE$, the online branch yields
\[
R_T\le C_{\mathrm{SL}}\sqrt{Td\,L_T^3}.
\]
\end{proposition}

\begin{proof}
The standard SupLinUCB counting argument uses only the following ingredients:
\begin{enumerate}
\item the optimal action survives elimination at every layer;
\item every arm surviving a narrow layer is near-optimal;
\item stopping at a nonterminal layer certifies a large online width;
\item the layerwise online widths satisfy an elliptical-potential bound.
\end{enumerate}
In our wrapper these are supplied, respectively, by
Lemmas~\ref{lem:optimal-survives}, \ref{lem:survivor-quality},
\ref{lem:online-trigger}, and \ref{lem:online-potential}. The proof of
Theorem~1 in \cite{chu2011} is purely pathwise once those four ingredients hold, so the same dyadic
summation yields $R_T\le C_{\mathrm{SL}}\sqrt{Td\,L_T^3}$ on $\cE$.
\end{proof}

\section{Proof of Theorem~\ref{thm:main}}

We now prove the pooled part of the theorem in full detail.

For each layer let
\[
Q_\ell:=\{t\in[T]:\ell_t=\ell\},
\qquad
A_\ell^{\mathrm{fin}}
:=
\sum_{t\in Q_\ell}x_{t,a_t}x_{t,a_t}^\top.
\]
Define
\[
\Lambda_\ell
:=
\log\frac{\det(A_\ell^{\mathrm{fin}}+G_{\mathrm{off}})}{\det(G_{\mathrm{off}})},
\qquad
\widetilde\Lambda_T
:=
\sum_{\ell=0}^{\lceil\log_2 T\rceil}\Lambda_\ell,
\qquad
\widetilde\Psi_T
:=
\sum_{t=1}^T \psi_{t,\ell_t}(x_{t,a_t}).
\]
Also set
\[
\delta_{\ell,\min}^{\mathrm{pool}}
:=
\min_{t\le T}\delta_{t,\ell}^{\mathrm{pool}},
\qquad
\gamma_\ell^{\mathrm{fin}}
:=
\sigma\sqrt{2\log\frac{\det(I+A_\ell^{\mathrm{fin}})^{1/2}}{\delta_{\ell,\min}^{\mathrm{pool}}}}
+S,
\]
\[
\delta_{\min}^{\mathrm{pool}}
:=
\min_{t,\ell}\delta_{t,\ell}^{\mathrm{pool}},
\qquad
\gamma_\star
:=
\sigma\sqrt{d\log(1+T)+2\log(1/\delta_{\min}^{\mathrm{pool}})}
+S,
\]
so that $\beta_\star=\beta_{\mathrm{off}}+\gamma_\star$.

\begin{lemma}[Layerwise pooled elliptical potential]
\label{lem:pooled-potential}
For every layer $\ell$,
\[
\sum_{t\in Q_\ell}\|x_{t,a_t}\|_{(A_{t,\ell}+G_{\mathrm{off}})^{-1}}^2
\le
2\log\frac{\det(A_\ell^{\mathrm{fin}}+G_{\mathrm{off}})}{\det(G_{\mathrm{off}})}.
\]
\end{lemma}

\begin{proof}
Enumerate $Q_\ell$ as $t_1<\cdots<t_{|Q_\ell|}$ and define
\[
W_{\ell,0}:=G_{\mathrm{off}},
\qquad
W_{\ell,j}:=G_{\mathrm{off}}+\sum_{i=1}^j x_{t_i,a_{t_i}}x_{t_i,a_{t_i}}^\top.
\]
Then $W_{\ell,j-1}=A_{t_j,\ell}+G_{\mathrm{off}}$ and
$W_{\ell,|Q_\ell|}=A_\ell^{\mathrm{fin}}+G_{\mathrm{off}}$. The matrix-determinant lemma yields
\[
\det(W_{\ell,j})
=
\det(W_{\ell,j-1})
\left(
1+\|x_{t_j,a_{t_j}}\|_{W_{\ell,j-1}^{-1}}^2
\right).
\]
Taking logarithms and summing,
\[
\log\frac{\det(A_\ell^{\mathrm{fin}}+G_{\mathrm{off}})}{\det(G_{\mathrm{off}})}
=
\sum_{j=1}^{|Q_\ell|}
\log\left(1+\|x_{t_j,a_{t_j}}\|_{W_{\ell,j-1}^{-1}}^2\right).
\]
Since $G_{\mathrm{off}}\succeq I$ and $W_{\ell,j-1}\succeq G_{\mathrm{off}}$, we have
$W_{\ell,j-1}^{-1}\preceq I$, hence for $\|x_{t_j,a_{t_j}}\|_2\le 1$,
\[
\|x_{t_j,a_{t_j}}\|_{W_{\ell,j-1}^{-1}}^2\le 1.
\]
Therefore $\log(1+u)\ge u/2$ on this range, and the claim follows.
\end{proof}

\begin{corollary}[Pooled variance accumulation]
\label{cor:pooled-variance}
We have
\[
\sum_{t=1}^T \|x_{t,a_t}\|_{(A_{t,\ell_t}+G_{\mathrm{off}})^{-1}}
\le
\sqrt{2T\,\widetilde\Lambda_T}.
\]
\end{corollary}

\begin{proof}
For each layer,
\[
\sum_{t\in Q_\ell}\|x_{t,a_t}\|_{(A_{t,\ell}+G_{\mathrm{off}})^{-1}}
\le
\sqrt{|Q_\ell|}
\left(
\sum_{t\in Q_\ell}\|x_{t,a_t}\|_{(A_{t,\ell}+G_{\mathrm{off}})^{-1}}^2
\right)^{1/2}
\]
by Cauchy--Schwarz. Apply Lemma~\ref{lem:pooled-potential}, then sum over $\ell$ and apply
Cauchy--Schwarz again across layers.
\end{proof}

\begin{proof}[Proof of Theorem~\ref{thm:main}]
On $\cE$, Proposition~\ref{prop:online-fallback} gives the fallback term
$C_{\mathrm{SL}}\sqrt{Td\,L_T^3}$. It therefore remains to prove the pooled term.

By Lemma~\ref{lem:stopping-regret},
\[
R_T
\le
8\sum_{t=1}^T \min\left\{1,\mathrm{rad}_{t,\ell_t}^{\mathrm{pool}}(x_{t,a_t})\right\}
\le
8\sum_{t=1}^T \mathrm{rad}_{t,\ell_t}^{\mathrm{pool}}(x_{t,a_t}),
\]
since $\min\{1,r\}\le r$ for $r\ge 0$. Expanding the pooled radius,
\[
R_T
\le
8\sum_{\ell=0}^{\lceil\log_2 T\rceil}\sum_{t\in Q_\ell}
\bigl(\gamma_{t,\ell_t}+\beta_{\mathrm{off}}\bigr)
\|x_{t,a_t}\|_{(A_{t,\ell_t}+G_{\mathrm{off}})^{-1}}
+8\rho\sum_{t=1}^T \psi_{t,\ell_t}(x_{t,a_t}).
\]
For every $t\in Q_\ell$, we have $\delta_{t,\ell}^{\mathrm{pool}}\ge \delta_{\ell,\min}^{\mathrm{pool}}$
and $V_{t,\ell}\preceq I+A_\ell^{\mathrm{fin}}$, so $\gamma_{t,\ell}\le \gamma_\ell^{\mathrm{fin}}$.
Therefore
\[
R_T
\le
8\sum_{\ell=0}^{\lceil\log_2 T\rceil}
\bigl(\beta_{\mathrm{off}}+\gamma_\ell^{\mathrm{fin}}\bigr)
\sum_{t\in Q_\ell}\|x_{t,a_t}\|_{(A_{t,\ell}+G_{\mathrm{off}})^{-1}}
+ 8\rho\,\widetilde\Psi_T.
\]
For each layer, Cauchy--Schwarz and Lemma~\ref{lem:pooled-potential} give
\[
\sum_{t\in Q_\ell}\|x_{t,a_t}\|_{(A_{t,\ell}+G_{\mathrm{off}})^{-1}}
\le
\sqrt{|Q_\ell|}
\left(
\sum_{t\in Q_\ell}\|x_{t,a_t}\|_{(A_{t,\ell}+G_{\mathrm{off}})^{-1}}^2
\right)^{1/2}
\le
\sqrt{2|Q_\ell|\Lambda_\ell}.
\]
Substituting this into the previous display proves the theorem's first pooled bound:
\[
R_T
\le
8\sum_{\ell=0}^{\lceil\log_2 T\rceil}
\bigl(\beta_{\mathrm{off}}+\gamma_\ell^{\mathrm{fin}}\bigr)\sqrt{2|Q_\ell|\Lambda_\ell}
+ 8\rho\,\widetilde\Psi_T.
\]
For the coarser simplification, note that $\delta_{\ell,\min}^{\mathrm{pool}}\ge\delta_{\min}^{\mathrm{pool}}$
and
\[
\det(I+A_\ell^{\mathrm{fin}})\le \left(1+\frac{T}{d}\right)^d\le (1+T)^d,
\]
so every $\gamma_\ell^{\mathrm{fin}}$ is at most $\gamma_\star$. Hence
\[
\sum_{\ell=0}^{\lceil\log_2 T\rceil}
\bigl(\beta_{\mathrm{off}}+\gamma_\ell^{\mathrm{fin}}\bigr)\sqrt{2|Q_\ell|\Lambda_\ell}
\le
\beta_\star
\sum_{\ell=0}^{\lceil\log_2 T\rceil}\sqrt{2|Q_\ell|\Lambda_\ell}.
\]
Applying Cauchy--Schwarz across layers and using $\sum_\ell |Q_\ell|=T$ yields
\[
\sum_{\ell=0}^{\lceil\log_2 T\rceil}\sqrt{2|Q_\ell|\Lambda_\ell}
\le
\sqrt{2T\,\widetilde\Lambda_T},
\]
which proves the theorem's second pooled bound. Both the fallback term and the pooled terms hold on
the same event $\cE$, so taking the minimum of the two completes the proof.
\end{proof}

\section{Proof of Proposition~\ref{prop:pooled-geometry}}

\begin{proof}
Write $A:=A_{t,\ell}$, $G:=G_{\mathrm{off}}$, and $M:=M_{\mathrm{shift}}$. By definition,
\[
\psi_{t,\ell}(x)^2
=
x^\top(A+G)^{-1}GM^{-1}G(A+G)^{-1}x.
\]
Under the matrix condition $GM^{-1}G\preceq c_{\mathrm{shift}}G$,
\[
\psi_{t,\ell}(x)^2
\le
c_{\mathrm{shift}}\,x^\top(A+G)^{-1}G(A+G)^{-1}x.
\]
Since $G\preceq A+G$, we have
\[
(A+G)^{-1}G(A+G)^{-1}\preceq (A+G)^{-1},
\]
and therefore
\[
\psi_{t,\ell}(x)^2
\le
c_{\mathrm{shift}}\|x\|_{(A+G)^{-1}}^2.
\]
Summing over the realized path and then using Lemma~\ref{lem:pooled-potential} layer by layer gives
\[
\sum_{t=1}^T \psi_{t,\ell_t}(x_{t,a_t})^2
\le
2c_{\mathrm{shift}}\widetilde\Lambda_T.
\]
Finally, Cauchy--Schwarz yields
\[
\widetilde\Psi_T
=
\sum_{t=1}^T \psi_{t,\ell_t}(x_{t,a_t})
\le
\sqrt{T\sum_{t=1}^T \psi_{t,\ell_t}(x_{t,a_t})^2}
\le
\sqrt{2c_{\mathrm{shift}}T\,\widetilde\Lambda_T}.
\]
Substituting this into Theorem~\ref{thm:main} gives the displayed bound.
\end{proof}

\begin{proof}[Proof of Corollary~\ref{cor:effective-dim}]
Proposition~\ref{prop:pooled-geometry} gives
\[
R_T
\le
8\beta_\star\sqrt{2T\,\widetilde\Lambda_T}
+
8\rho\sqrt{2 c_{\mathrm{shift}} T\,\widetilde\Lambda_T}.
\]
Using $\widetilde\Lambda_T \le d_{\mathrm{eff}}\log(1+T)$ and factoring the common term yields
\[
R_T
\le
8\bigl(\beta_\star+\rho\sqrt{c_{\mathrm{shift}}}\bigr)
\sqrt{2T\,d_{\mathrm{eff}}\log(1+T)},
\]
which is exactly the claim.
\end{proof}

\section{Proof of Theorem~\ref{thm:lower}}

\begin{proof}
Fix any possibly randomized policy in the oracle model where $\theta^\dagger$ is revealed before
round~$1$. We embed a hard $(d-1)$-armed Bernoulli bandit problem into the linear contextual class.
Throughout the construction the offline sample can be arbitrary, because the theorem only strengthens
the learner by additionally revealing $\theta^\dagger$ itself. We prove the claim under the numerical
conditions $d\ge 9$ and $T\ge d^2$, which are exactly the regime stated in
Theorem~\ref{thm:lower}. Fix the baseline
\[
\theta^\dagger:=\frac{1}{2\sqrt{2}}e_1.
\]
For each $j\in[d-1]$, define
\[
\theta^{(j)}:=\theta^\dagger+\rho e_{j+1}.
\]
Then
\[
\|\theta^{(j)}-\theta^\dagger\|_2=\rho,
\]
so every instance satisfies the isotropic certificate.

Choose the action set
\[
x_a:=\frac{e_1+e_{a+1}}{\sqrt{2}},
\qquad
a\in[d-1].
\]
This uses only $d-1$ arms, so it is admissible when $K\ge d-1$.
Under instance $j$,
\[
x_a^\top\theta^{(j)}
=
\frac14+\frac{\rho}{\sqrt{2}}\mathbf{1}\{a=j\},
\]
and we instantiate rewards as Bernoulli random variables with these means. Thus arm $j$ is uniquely
optimal with gap $\rho/\sqrt{2}$. Let $P_j$ denote the law of the interaction
under instance $j$, and let $P_0$ denote the null instance with parameter $\theta^\dagger$, under
which all arms have mean $1/4$.

Let
\[
N_j:=\sum_{t=1}^T \mathbf{1}\{a_t=j\}
\]
be the number of pulls of arm $j$. Choose $j^\star$ minimizing $\E_0[N_j]$. Since
$\sum_{j=1}^{d-1}N_j=T$, we have
\[
\E_0[N_{j^\star}]\le \frac{T}{d-1}.
\]

\paragraph{Small-shift regime.}
Assume first that
\[
\rho\le \frac18\sqrt{\frac{d-1}{T}}.
\]
Since $T\ge d^2$ and $d\ge 9$, this implies $\rho\le 1/4$. Therefore
\[
\|\theta^{(j)}\|_2^2=\frac18+\rho^2\le 1\le S,
\]
so the construction respects the parameter-norm assumption.
Define the event
\[
E:=\{N_{j^\star}>T/2\}.
\]
By Markov's inequality,
\[
\Prb_0(E)\le \frac{2}{d-1}.
\]
Next compute the KL divergence between the null and shifted reward laws on a pull of arm $j^\star$.
The null mean is $1/4$, while the shifted mean is $1/4+\rho/\sqrt{2}$. Using the standard Bernoulli
bound $\mathrm{kl}(p,q)\le (q-p)^2/(p(1-q))$,
\[
\mathrm{kl}\!\left(\frac14,\frac14+\frac{\rho}{\sqrt{2}}\right)
\le
\frac{(\rho/\sqrt{2})^2}{(1/4)(3/4-\rho/\sqrt{2})}
\le 4\rho^2.
\]
Since only pulls of arm $j^\star$ distinguish $P_0$ from $P_{j^\star}$,
\[
\mathrm{KL}(P_0,P_{j^\star})
=
\E_0[N_{j^\star}]
\cdot
\mathrm{kl}\!\left(\frac14,\frac14+\frac{\rho}{\sqrt{2}}\right)
\le
\frac{4\rho^2T}{d-1}
\le \frac{1}{16}.
\]
Apply the Bretagnolle--Huber inequality:
\[
\Prb_{j^\star}(E^c)+\Prb_0(E)\ge \frac12 e^{-\mathrm{KL}(P_0,P_{j^\star})}.
\]
Using $d\ge 9$ and the bounds above,
\[
\Prb_{j^\star}(E^c)
\ge
\frac12 e^{-1/16}-\frac{2}{d-1}
\ge \frac15.
\]
On $E^c$, the optimal arm is pulled at most $T/2$ times, so at least $T/2$ rounds incur gap
$\rho/\sqrt{2}$. Therefore
\[
\E_{j^\star}[R_T]
\ge
\frac{\rho}{\sqrt{2}}\cdot \frac{T}{2}\cdot \Prb_{j^\star}(E^c)
\ge
\frac{\rho T}{10\sqrt{2}}.
\]

\paragraph{Large-shift regime.}
Now suppose
\[
\rho>\frac18\sqrt{\frac{d-1}{T}}.
\]
Set
\[
\rho_0:=\frac18\sqrt{\frac{d-1}{T}}.
\]
By $T\ge d^2$ and $d\ge 9$, we have $\rho_0\le 1/4$, so the same construction is admissible with
$\rho_0$ in place of $\rho$.
Every instance allowed under $\rho_0$ is also allowed under $\rho$, so the lower bound from the
small-shift regime applies with $\rho_0$:
\[
\sup_{I}\E_I[R_T]
\ge
c_1 \rho_0 T
=
\frac{c_1}{8}\sqrt{(d-1)T}
\ge
c_2\sqrt{dT}.
\]
Combining the two regimes yields
\[
\sup_I \E_I[R_T]\ge c\,\min\{\rho T,\sqrt{dT}\}
\]
for a universal constant $c>0$.
\end{proof}

\section{Diagonal specialization and connection to MIN-UCB}
\label{app:diagonal-specialization}

The following statements isolate when the linear pooled score reduces to the familiar arm-wise
template of scalar MIN-UCB \citep{cheung2024}. They are not used in the proof of Theorem~\ref{thm:main}.

\begin{proposition}[Diagonal specialization]
\label{prop:diagonal}
Assume the action vectors form an orthonormal basis and that $G_{\mathrm{off}}$ and
$M_{\mathrm{shift}}$ are diagonal in that same basis. After rotating to this basis, write the
actions as $\{e_a\}$, set
\[
n_a:=e_a^\top G_{\mathrm{off}}e_a,
\qquad
v_a:=\frac{\rho}{\sqrt{e_a^\top M_{\mathrm{shift}}e_a}},
\qquad
\hat\mu^{\mathrm{pool}}_{t,\ell}(a):=e_a^\top\hat\theta^{\mathrm{pool}}_{t,\ell},
\]
and let $N_{t,\ell}(a)$ denote the number of times arm $a$ has been routed
to layer $\ell$ before round $t$. Then the layerwise pooled UCB becomes arm-wise:
\[
U^{\mathrm{pool}}_{t,\ell}(a)
=
\hat\mu^{\mathrm{pool}}_{t,\ell}(a)
+ \frac{\gamma_{t,\ell}+\beta_{\mathrm{off}}}{\sqrt{N_{t,\ell}(a)+n_a}}
+ \frac{n_a}{N_{t,\ell}(a)+n_a}v_a,
\]
with pseudo-counts $n_a$ and directional bias budgets $v_a$. Hence the scalar MIN-UCB
bias-contraction structure is recovered as a special case of the linear construction.
\end{proposition}

\begin{corollary}[Arm-wise activation on the diagonal class]
\label{cor:diagonal-activation}
Under the assumptions of Proposition~\ref{prop:diagonal}, the online radius on arm $a$ is
\[
\mathrm{rad}^{\mathrm{on}}_{t,\ell}(e_a)
=
\frac{\beta^{\mathrm{on}}_{t,\ell}}{\sqrt{N_{t,\ell}(a)+1}},
\]
whereas the pooled radius is
\[
\mathrm{rad}^{\mathrm{pool}}_{t,\ell}(e_a)
=
\frac{\gamma_{t,\ell}+\beta_{\mathrm{off}}}{\sqrt{N_{t,\ell}(a)+n_a}}
+
\frac{n_a}{N_{t,\ell}(a)+n_a}v_a.
\]
Consequently, if
\[
\frac{\beta^{\mathrm{on}}_{t,\ell}}{\sqrt{N_{t,\ell}(a)+1}}
-
\frac{\gamma_{t,\ell}+\beta_{\mathrm{off}}}{\sqrt{N_{t,\ell}(a)+n_a}}
-
\frac{n_a}{N_{t,\ell}(a)+n_a}v_a
\ge
\left|e_a^\top\bigl(\hat\theta^{\mathrm{pool}}_{t,\ell}-\hat\theta^{\mathrm{on}}_{t,\ell}\bigr)\right|,
\]
then the aggregated UCB/LCB pair on arm $a$ coincides with the pooled branch.
\end{corollary}

Proposition~\ref{prop:diagonal} is a \emph{structural} statement, not an algorithmic identification.
It does not assert that Ellipsoidal-MINUCB reduces to the original MIN-UCB policy. It asserts that,
when $G_{\mathrm{off}}$ and $M_{\mathrm{shift}}$ align with the action basis, the layerwise pooled
UCB admits the same pseudo-count and bias-budget decomposition as scalar MIN-UCB. In that regime the
familiar bias--contraction pattern is recovered as a specialization of the linear pooled score, not
as an independent design choice. Corollary~\ref{cor:diagonal-activation} makes the same point at the
decision level: larger pseudo-counts $n_a$ and smaller bias budgets $v_a$ are exactly what makes the
pooled branch activate on a given arm.

\section{Proof of Proposition~\ref{prop:diagonal}}

\begin{proof}
Assume the action vectors form an orthonormal basis and both $G_{\mathrm{off}}$ and
$M_{\mathrm{shift}}$ are diagonal in the same basis. After the orthogonal change of coordinates that
sends each action vector to a canonical basis vector, we may work directly with $x_{t,a}=e_a$.

Let
\[
A_{t,\ell}:=\sum_{s\in\cH_{t,\ell}} x_{s,a_s}x_{s,a_s}^\top
\]
be the layerwise online Gram matrix, and let
\[
N_{t,\ell}(a):=\sum_{s\in\cH_{t,\ell}}\mathbf{1}\{a_s=a\}.
\]
Because pulling arm $a$ only updates coordinate $a$, we
have
\[
A_{t,\ell} e_a = N_{t,\ell}(a)e_a,
\qquad
G_{\mathrm{off}}e_a = n_a e_a,
\qquad
M_{\mathrm{shift}}e_a = m_a e_a.
\]
Therefore
\[
(A_{t,\ell}+G_{\mathrm{off}})e_a=(N_{t,\ell}(a)+n_a)e_a,
\]
so the pooled estimator on coordinate $a$ is
\[
e_a^\top \hat\theta_{t,\ell}^{\mathrm{pool}}
=
\frac{\sum_{s\in\cH_{t,\ell}:\,a_s=a} r_s + n_a\,e_a^\top\hat\theta_{\mathrm{off}}}
{N_{t,\ell}(a)+n_a}
=:
\hat\mu_{t,\ell}^{\mathrm{pool}}(a).
\]
This proves the coordinate-wise form of the pooled mean.

The statistical part of the radius is equally explicit:
\[
\|e_a\|_{(A_{t,\ell}+G_{\mathrm{off}})^{-1}}
=
\frac{1}{\sqrt{N_{t,\ell}(a)+n_a}}.
\]
For the shift term,
\[
\psi_{t,\ell}(e_a)
=
\left\|
M_{\mathrm{shift}}^{-1/2}G_{\mathrm{off}}(A_{t,\ell}+G_{\mathrm{off}})^{-1}e_a
\right\|_2
=
\left\|
M_{\mathrm{shift}}^{-1/2}\frac{n_a}{N_{t,\ell}(a)+n_a}e_a
\right\|_2
=
\frac{n_a}{N_{t,\ell}(a)+n_a}\frac{1}{\sqrt{m_a}}.
\]
Multiplying by $\rho$ gives
\[
\rho\,\psi_{t,\ell}(e_a)
=
\frac{n_a}{N_{t,\ell}(a)+n_a}\frac{\rho}{\sqrt{m_a}}
=
\frac{n_a}{N_{t,\ell}(a)+n_a}v_a.
\]
Substituting the last two displays into the pooled score yields exactly
\[
U_{t,\ell}^{\mathrm{pool}}(a)
=
\hat\mu_{t,\ell}^{\mathrm{pool}}(a)
+ \frac{\gamma_{t,\ell}+\beta_{\mathrm{off}}}{\sqrt{N_{t,\ell}(a)+n_a}}
+ \frac{n_a}{N_{t,\ell}(a)+n_a}v_a.
\]
Thus the diagonal specialization recovers the same bias-contraction template as scalar MIN-UCB, with
$n_a$ playing the role of pseudo-counts and $v_a$ the role of arm-wise bias budgets.
\end{proof}

\begin{proof}[Proof of Corollary~\ref{cor:diagonal-activation}]
Under the diagonal assumptions, the online Gram matrix satisfies
\[
V_{t,\ell}e_a=(N_{t,\ell}(a)+1)e_a,
\]
so
\[
\mathrm{rad}^{\mathrm{on}}_{t,\ell}(e_a)
=
\beta^{\mathrm{on}}_{t,\ell}\|e_a\|_{V_{t,\ell}^{-1}}
=
\frac{\beta^{\mathrm{on}}_{t,\ell}}{\sqrt{N_{t,\ell}(a)+1}}.
\]
The formula for $\mathrm{rad}^{\mathrm{pool}}_{t,\ell}(e_a)$ is exactly the one derived in
Proposition~\ref{prop:diagonal}. Therefore
\[
\Delta_{t,\ell}(e_a)
=
\mathrm{rad}^{\mathrm{on}}_{t,\ell}(e_a)-\mathrm{rad}^{\mathrm{pool}}_{t,\ell}(e_a)
\]
is the left-hand side of the displayed condition. The conclusion then follows immediately from
Proposition~\ref{prop:helpfulness}.
\end{proof}

\section{Directional helpfulness and pooled-branch activation}
\label{app:directional-helpfulness}

Section~\ref{sec:algorithm} defines $\Delta_{t,\ell}(x)$, $h_{\mathrm{off}}(x)$, and the pooled versus
online radii. The next two results record when the pooled confidence interval nests inside the online
one along a set of directions, and a sufficient matrix-based screening inequality.

\begin{proposition}[Helpfulness and pooled-branch activation]
\label{prop:helpfulness}
Fix a round-layer pair $(t,\ell)$ and a set $\mathcal{X} \subseteq \R^d$. Suppose that for every
$x \in \mathcal{X}$,
\[
\Delta_{t,\ell}(x)
\ge
\left|
x^{\top}\bigl(\hat\theta^{\mathrm{pool}}_{t,\ell}-\hat\theta^{\mathrm{on}}_{t,\ell}\bigr)
\right|.
\]
Then every action $a$ with $x_{t,a} \in \mathcal{X}$ satisfies
\[
U^{\mathrm{pool}}_{t,\ell}(a)\le U^{\mathrm{on}}_{t,\ell}(a),
\qquad
L^{\mathrm{pool}}_{t,\ell}(a)\ge L^{\mathrm{on}}_{t,\ell}(a).
\]
Consequently the aggregated UCB and LCB coincide with the pooled UCB and pooled LCB on $\mathcal{X}$:
\[
U^{\min}_{t,\ell}(a)=U^{\mathrm{pool}}_{t,\ell}(a),
\qquad
L^{\max}_{t,\ell}(a)=L^{\mathrm{pool}}_{t,\ell}(a).
\]
\end{proposition}

\begin{corollary}[Screening condition for pooled activation]
\label{cor:helpfulness-screen}
Define
\[
\kappa_{\mathrm{shift}}
:=
\|M_{\mathrm{shift}}^{-1/2}G_{\mathrm{off}}^{1/2}\|_{\mathrm{op}},
\]
so that
\[
G_{\mathrm{off}}M_{\mathrm{shift}}^{-1}G_{\mathrm{off}}
\preceq
\kappa_{\mathrm{shift}}^2 G_{\mathrm{off}}.
\]
For every round-layer pair $(t,\ell)$ and direction $x\in\R^d$,
\[
\Delta_{t,\ell}(x)
\ge
\beta^{\mathrm{on}}_{t,\ell}\|x\|_{V_{t,\ell}^{-1}}
-
\bigl(\gamma_{t,\ell}+\beta_{\mathrm{off}}+\rho\kappa_{\mathrm{shift}}\bigr)
\|x\|_{(A_{t,\ell}+G_{\mathrm{off}})^{-1}}.
\]
Consequently, if there exists $\varepsilon\ge 0$ such that for every $x\in\mathcal{X}$,
\[
\beta^{\mathrm{on}}_{t,\ell}\|x\|_{V_{t,\ell}^{-1}}
\ge
\bigl(\gamma_{t,\ell}+\beta_{\mathrm{off}}+\rho\kappa_{\mathrm{shift}}\bigr)
\|x\|_{(A_{t,\ell}+G_{\mathrm{off}})^{-1}}
+
\varepsilon
\]
and
\[
\left|
x^{\top}\bigl(\hat\theta^{\mathrm{pool}}_{t,\ell}-\hat\theta^{\mathrm{on}}_{t,\ell}\bigr)
\right|
\le \varepsilon,
\]
then the aggregated UCB/LCB pair coincides with the pooled branch on $\mathcal{X}$.
\end{corollary}

\begin{proof}[Proof of Proposition~\ref{prop:helpfulness}]
Fix $x \in \mathcal{X}$ and an action $a$ with $x_{t,a}=x$. By definition,
\[
U^{\mathrm{on}}_{t,\ell}(a)-U^{\mathrm{pool}}_{t,\ell}(a)
=
x^{\top}(\hat\theta^{\mathrm{on}}_{t,\ell}-\hat\theta^{\mathrm{pool}}_{t,\ell})
+
\Delta_{t,\ell}(x),
\]
so
\[
U^{\mathrm{on}}_{t,\ell}(a)\ge U^{\mathrm{pool}}_{t,\ell}(a)
\qquad\Longleftrightarrow\qquad
x^{\top}(\hat\theta^{\mathrm{pool}}_{t,\ell}-\hat\theta^{\mathrm{on}}_{t,\ell})
\le
\Delta_{t,\ell}(x).
\]
Similarly, with symmetric LCBs,
\[
L^{\mathrm{pool}}_{t,\ell}(a)-L^{\mathrm{on}}_{t,\ell}(a)
=
x^{\top}(\hat\theta^{\mathrm{pool}}_{t,\ell}-\hat\theta^{\mathrm{on}}_{t,\ell})
+
\Delta_{t,\ell}(x),
\]
so
\[
L^{\mathrm{pool}}_{t,\ell}(a)\ge L^{\mathrm{on}}_{t,\ell}(a)
\qquad\Longleftrightarrow\qquad
x^{\top}(\hat\theta^{\mathrm{pool}}_{t,\ell}-\hat\theta^{\mathrm{on}}_{t,\ell})
\ge
-\Delta_{t,\ell}(x).
\]
The assumption of the proposition is exactly the conjunction of these two inequalities. Therefore the
pooled UCB--LCB pair is nested inside the online UCB--LCB pair on every action whose feature lies
in $\mathcal{X}$, and the branch aggregation rule reduces to
\[
U^{\min}_{t,\ell}(a)=U^{\mathrm{pool}}_{t,\ell}(a),
\qquad
L^{\max}_{t,\ell}(a)=L^{\mathrm{pool}}_{t,\ell}(a).
\]
\end{proof}

\begin{proof}[Proof of Corollary~\ref{cor:helpfulness-screen}]
By definition,
\[
\Delta_{t,\ell}(x)
=
\beta^{\mathrm{on}}_{t,\ell}\|x\|_{V_{t,\ell}^{-1}}
-
\bigl(\gamma_{t,\ell}+\beta_{\mathrm{off}}\bigr)\|x\|_{(A_{t,\ell}+G_{\mathrm{off}})^{-1}}
-
\rho\,\psi_{t,\ell}(x).
\]
\[
G_{\mathrm{off}}M_{\mathrm{shift}}^{-1}G_{\mathrm{off}}
=
G_{\mathrm{off}}^{1/2}
\bigl(G_{\mathrm{off}}^{1/2}M_{\mathrm{shift}}^{-1}G_{\mathrm{off}}^{1/2}\bigr)
G_{\mathrm{off}}^{1/2}
\preceq
\kappa_{\mathrm{shift}}^2 G_{\mathrm{off}}.
\]
Therefore, exactly as in the proof of Proposition~\ref{prop:pooled-geometry},
\[
\psi_{t,\ell}(x)^2
\le
\kappa_{\mathrm{shift}}^2
x^\top(A_{t,\ell}+G_{\mathrm{off}})^{-1}
G_{\mathrm{off}}
(A_{t,\ell}+G_{\mathrm{off}})^{-1}x
\le
\kappa_{\mathrm{shift}}^2
\|x\|_{(A_{t,\ell}+G_{\mathrm{off}})^{-1}}^2,
\]
where the last step uses
\[
(A_{t,\ell}+G_{\mathrm{off}})^{-1}G_{\mathrm{off}}(A_{t,\ell}+G_{\mathrm{off}})^{-1}
\preceq
(A_{t,\ell}+G_{\mathrm{off}})^{-1}.
\]
Hence
\[
\psi_{t,\ell}(x)
\le
\kappa_{\mathrm{shift}}
\|x\|_{(A_{t,\ell}+G_{\mathrm{off}})^{-1}}.
\]
Substituting this bound into the definition of $\Delta_{t,\ell}(x)$ gives
\[
\Delta_{t,\ell}(x)
\ge
\beta^{\mathrm{on}}_{t,\ell}\|x\|_{V_{t,\ell}^{-1}}
-
\bigl(\gamma_{t,\ell}+\beta_{\mathrm{off}}+\rho\kappa_{\mathrm{shift}}\bigr)
\|x\|_{(A_{t,\ell}+G_{\mathrm{off}})^{-1}}.
\]
Hence the two displayed assumptions imply
\[
\Delta_{t,\ell}(x)\ge
\left|
x^\top(\hat\theta^{\mathrm{pool}}_{t,\ell}-\hat\theta^{\mathrm{on}}_{t,\ell})
\right|
\]
for every $x\in\mathcal{X}$. Proposition~\ref{prop:helpfulness} then yields the claim.
\end{proof}

\section{Data-driven directional shift certificates: details and proofs (Section~\ref{sec:epoch-wise-ell-minucb})}
\label{app:epoch-learned-proofs}

\subsection{Pooled width, certificate validity, algorithm, and doubling refinement}
\label{app:epoch-dd-details}

On rounds $t\in\{\tau_k,\ldots,\tau_{k+1}-1\}$ one replaces
$\rho\,\psi_{t,\ell}$ of the main text by $\widehat\rho_k\,\widehat\psi_{k,t,\ell}$ with
\begin{equation}
\label{eq:epoch-psi}
\widehat\psi_{k,t,\ell}(x)
:=
\left\|
\widehat M_k^{-1/2}G_{\mathrm{off}}(A_{t,\ell}+G_{\mathrm{off}})^{-1}x
\right\|_2
\end{equation}
and
\begin{equation}
\label{eq:epoch-pool-rad}
\widehat{\mathrm{rad}}^{\mathrm{pool,ep}}_{t,\ell}(x)
:=
\bigl(\gamma_{t,\ell}+\beta_{\mathrm{off}}\bigr)\|x\|_{(A_{t,\ell}+G_{\mathrm{off}})^{-1}}
+\widehat\rho_k\,\widehat\psi_{k,t,\ell}(x).
\end{equation}

\begin{theorem}[Validity of the learned parallel-sum certificate]
\label{thm:epoch-parallel-cert-valid}
Suppose the standard offline ridge and epoch-wise online events hold, i.e.\
\(
\|\theta^\dagger-\hat\theta_{\mathrm{off}}\|_{G_{\mathrm{off}}}\le\beta_{\mathrm{off}}(\delta_{\mathrm{off}})
\)
and, for every~$k$,
\(
\|\theta_*-\hat\theta_k^{\mathrm{on}}\|_{G_k^{\mathrm{on}}}\le\beta_k^{\mathrm{on}}(\delta_k)
\).
If
\(
\delta_{\mathrm{off}}+\sum_{k=1}^{K_{\mathrm{ep}}}\delta_k
\le\delta_{\mathrm{cert}}
\)
then, with probability at least $1-\delta_{\mathrm{cert}}$,
\[
\|\theta_*-\theta^\dagger\|_{\widehat M_k}
\le
\widehat\rho_k
\qquad
\forall k\in\{1,\ldots,K_{\mathrm{ep}}\}.
\]
\end{theorem}

\paragraph{Remark.}
The epoch-wise min/max layer shell is the same as in the main text
(Algorithm~\ref{alg:epoch-ell-minucb} there; shift routing in \eqref{eq:epoch-psi}--\eqref{eq:epoch-pool-rad} above).

\paragraph{Doubling epochs and a closed-form bound.}
A default is
$K_{\mathrm{ep}}:=\lfloor\log_2 T\rfloor+1$,
\(
\tau_k:=2^{k-1}
\),
\(
\tau_{K_{\mathrm{ep}}+1}:=T+1
\).
To combine Theorems~\ref{thm:epoch-parallel-cert-valid}--\ref{thm:epoch-parallel-regret} with
closed-form radii, split
\(
\delta_{\mathrm{off}}:=\delta_{\mathrm{cert}}/2
\)
and
\(
\delta_k:=\delta_{\mathrm{cert}}/(2K_{\mathrm{ep}})
\)
and set
\[
\beta_k^{\mathrm{on}}
:=
\sigma\sqrt{
d\log(1{+}\tau_k)
+2\log(2K_{\mathrm{ep}}/\delta_{\mathrm{cert}})}
+S,
\qquad
\beta_{\mathrm{off}}^{\mathrm{cert}}
:=
\sigma\sqrt{
2\log\bigl(\det(G_{\mathrm{off}})^{1/2}/(\delta_{\mathrm{cert}}/2)\bigr)
}+S.
\]
In each epoch, with $\widehat\Delta_k$ and~$\widehat M_k$ built from~$D_{\mathrm{off}}$ and
online data before~$\tau_k$ (as in
Algorithm~\ref{alg:epoch-ell-minucb}), set
\(
\widehat\rho_k
:=
\|\widehat\Delta_k\|_{\widehat M_k}
+\beta_k^{\mathrm{on}}
+\beta_{\mathrm{off}}^{\mathrm{cert}}.
\)

\begin{theorem}[Doubling-epoch shift aggregation]
\label{thm:epoch-doubling-regret}
Under the doubling schedule, $\delta$-split, and
$(\widehat\rho_k,\widehat M_k)$ from the previous paragraph, define
$n_k:=\tau_{k+1}-\tau_k$,
\[
\widehat c_k
:=
\lambda_{\max}\bigl(
G_{\mathrm{off}}^{1/2}\widehat M_k^{-1}G_{\mathrm{off}}^{1/2}
\bigr),
\qquad
\mathcal S_{\mathrm{ep}}
:=
\sum_{k=1}^{K_{\mathrm{ep}}} n_k\,\widehat\rho_k^2\,\widehat c_k.
\]
With probability at least $1-T^{-2}-\delta_{\mathrm{cert}}$, the regret satisfies
\[
R_T
\le
\min\left\{
C_{\mathrm{SL}}\sqrt{Td\,L_T^3},
\;
8\beta_\star\sqrt{2T\,\widetilde\Lambda_T}
+8\sqrt{2\,\widetilde\Lambda_T\,\mathcal S_{\mathrm{ep}}}
\right\},
\]
and also the same bound with
$8\beta_\star\sqrt{2T\,\widetilde\Lambda_T}$ replaced by the full layerwise statistical term
\(
8\sum_{\ell}
(\beta_{\mathrm{off}}+\gamma_\ell^{\mathrm{fin}})\sqrt{2|Q_\ell|\,\Lambda_\ell}
\),
where~$\beta_\star$ is as in Theorem~\ref{thm:main}.
\end{theorem}

\subsection{Proofs}

\begin{proof}[Proof of Theorem~\ref{thm:epoch-parallel-cert-valid}]
With probability at least $1-\delta_{\mathrm{off}}$,
\(
\|\theta^\dagger-\hat\theta_{\mathrm{off}}\|_{G_{\mathrm{off}}}\le\beta_{\mathrm{off}}(\delta_{\mathrm{off}})
\).
For each epoch~$k$, the estimator
$\hat\theta_k^{\mathrm{on}}$ uses only data strictly before~$\tau_k$; the self-normalized ridge
inequality at time~$\tau_k$ yields
\(
\|\theta_*-\hat\theta_k^{\mathrm{on}}\|_{G_k^{\mathrm{on}}}\le\beta_k^{\mathrm{on}}(\delta_k)
\)
on an event of probability at least~$1-\delta_k$ (in the predictable epoch case, the same
time-uniform bound or a union over~$t$ and evaluation at~$\tau_k$ applies). A union bound gives
simultaneous validity with probability at least $1-\delta_{\mathrm{cert}}$ when
\(
\delta_{\mathrm{off}}+\sum_k\delta_k\le\delta_{\mathrm{cert}}
\).

On this event, for fixed~$k$, the parallel-sum definition implies
\(
\widehat M_k\preceq G_k^{\mathrm{on}}
\)
and
\(
\widehat M_k\preceq G_{\mathrm{off}}
\)
because
\(
(G_k^{\mathrm{on}})^{-1}{+}G_{\mathrm{off}}^{-1}\succeq (G_k^{\mathrm{on}})^{-1}
\)
and the symmetric inequality for~$G_{\mathrm{off}}$. Hence, for all~$v$,
\(
\|v\|_{\widehat M_k}\le\|v\|_{G_k^{\mathrm{on}}}
\)
and
\(
\|v\|_{\widehat M_k}\le\|v\|_{G_{\mathrm{off}}}
\).
Decompose
\(
\theta_*-\theta^\dagger
=
\widehat\Delta_k
+(\theta_*-\hat\theta_k^{\mathrm{on}})
-(\theta^\dagger-\hat\theta_{\mathrm{off}})
\)
with
\(
\widehat\Delta_k:=\hat\theta_k^{\mathrm{on}}-\hat\theta_{\mathrm{off}}
\).
The triangle inequality in the~$\widehat M_k$ norm, together with the confidence events and
Loewner domination, gives
\[
\|\theta_*-\theta^\dagger\|_{\widehat M_k}
\le
\|\widehat\Delta_k\|_{\widehat M_k}
+\beta_k^{\mathrm{on}}(\delta_k)
+\beta_{\mathrm{off}}(\delta_{\mathrm{off}})
=\widehat\rho_k.
\]
Since~$k$ is arbitrary, the claim holds for all~$k$.
\end{proof}

\begin{proof}[Proof of Theorem~\ref{thm:epoch-parallel-regret}]
The online (SupLin) branch is unchanged, so the ordinary fallback regret term
$C_{\mathrm{SL}}\sqrt{Td\,L_T^3}$ and its proof are unchanged. For the pooled branch, on the event
of Theorem~\ref{thm:epoch-parallel-cert-valid},
\[
\|\theta_*-\theta^\dagger\|_{\widehat M_{k(t)}}
\le
\widehat\rho_{k(t)}
\qquad\forall t.
\]
The epoch start times are part of the prespecified (or past-measurable) rule, and
$(\widehat M_k,\widehat\rho_k)$ uses only data before~$\tau_k$; therefore the pair used in round~$t$
is $\cF_{t-1}$-measurable and the policy remains non-anticipatory, so the martingale and
self-normalized concentration events from the proof of Theorem~\ref{thm:main} are unchanged.
On the certificate event, for every round-$t$ queried direction~$x$,
\[
|x^\top(\theta_*-\theta^\dagger)|
\le
\widehat\rho_{k(t)}\|x\|_{\widehat M_{k(t)}^{-1}}.
\]
In the pooled confidence step (Lemma~\ref{lem:pooled-valid} in the main appendix proof), the fixed
shift width
\(
\rho\,\|M_{\mathrm{shift}}^{-1/2}G_{\mathrm{off}}(A_{t,\ell}{+}G_{\mathrm{off}})^{-1}x\|_2
\)
is therefore replaced by
$\widehat\rho_{k(t)}\bigl\|\widehat M_{k(t)}^{-1/2}G_{\mathrm{off}}(A_{t,\ell}{+}G_{\mathrm{off}})^{-1}x\bigr\|_2$,
i.e., $\widehat\rho_{k(t)}\widehat\psi_{k(t),t,\ell}(x)$. The UCB/LCB validity, elimination, and
stopping-layer arguments from the proof of Theorem~\ref{thm:main} then go through unchanged except
that the routed shift sum is~$\widetilde\Psi_T^{\mathrm{ep}}$, while the statistical (non-shift) part
of the pooled width still produces the
\(
8\sum_\ell
(\beta_{\mathrm{off}}{+}\gamma_\ell^{\mathrm{fin}})\sqrt{2|Q_\ell|\,\Lambda_\ell}
\)
term by the same pooled elliptical potential calculation. Intersecting the certificate event with
the original $1-T^{-2}$-probability event for the online, offline, and pooled self-normalized
events yields the stated probability and regret bound.
\end{proof}

\begin{proof}[Proof of Theorem~\ref{thm:epoch-doubling-regret}]
Start from Theorem~\ref{thm:epoch-parallel-regret}. For $t$ in epoch~$k$, write
$A:=A_{t,\ell_t}$ and $G:=G_{\mathrm{off}}$. By definition of~$\widehat\psi$,
\[
\widehat\psi_{k,t,\ell_t}(x_{t,a_t})^2
=
x_{t,a_t}^{\top}
(A+G)^{-1}
G\widehat M_k^{-1}G
(A+G)^{-1}
x_{t,a_t}.
\]
The choice
\(
\widehat c_k := \lambda_{\max}(G^{1/2}\widehat M_k^{-1}G^{1/2})
\)
is equivalent to
\(
G\widehat M_k^{-1}G\preceq \widehat c_k\,G
\)
in Loewner order, hence
\(
\widehat\psi_{k,t,\ell_t}(x_{t,a_t})^2
\le
\widehat c_k
\,x_{t,a_t}^{\top}
(A+G)^{-1}G(A+G)^{-1}x_{t,a_t}
\).
Since $G\preceq A+G$,
\(
(A+G)^{-1}G(A+G)^{-1}\preceq (A+G)^{-1}
\)
and
\[
\widehat\psi_{k,t,\ell_t}(x_{t,a_t})
\le
\sqrt{\widehat c_k}
\,\|x_{t,a_t}\|_{(A_{t,\ell_t}+G_{\mathrm{off}})^{-1}}.
\]
Therefore
\[
\widetilde\Psi_T^{\mathrm{ep}}
\le
\sum_{t=1}^T
\widehat\rho_{k(t)}\sqrt{\widehat c_{k(t)}}
\,\|x_{t,a_t}\|_{(A_{t,\ell_t}+G_{\mathrm{off}})^{-1}}.
\]
By Cauchy--Schwarz,
\[
\widetilde\Psi_T^{\mathrm{ep}}
\le
\Bigl(\sum_{t=1}^T \widehat\rho_{k(t)}^2\widehat c_{k(t)}\Bigr)^{1/2}
\Bigl(\sum_{t=1}^T \|x_{t,a_t}\|_{(A_{t,\ell_t}+G_{\mathrm{off}})^{-1}}^2\Bigr)^{1/2}.
\]
The first factor equals~$\sqrt{\mathcal S_{\mathrm{ep}}}$ because $(\widehat\rho_k,\widehat c_k)$ are
constant on each epoch. The second is at most~$\sqrt{2\,\widetilde\Lambda_T}$ by
Lemma~\ref{lem:pooled-potential} and the definition
\(
\widetilde\Lambda_T=\sum_\ell\Lambda_\ell
\)
in Theorem~\ref{thm:main}. Thus
\(
\widetilde\Psi_T^{\mathrm{ep}}\le \sqrt{2\,\widetilde\Lambda_T\,\mathcal S_{\mathrm{ep}}}
\).
Substitute into the minimum expression of Theorem~\ref{thm:epoch-parallel-regret} and use the
Cauchy--Schwarz step
\(
\sum_\ell
(\beta_{\mathrm{off}}+\gamma_\ell^{\mathrm{fin}})\sqrt{2|Q_\ell|\,\Lambda_\ell}
\le
\beta_\star\sqrt{2T\,\widetilde\Lambda_T}
\)
as in the proof of Theorem~\ref{thm:main} to obtain the two displayed bounds.
\end{proof}

\section{Additional Experiments}
\label{app:more-experiments}

The hyperparameters in Section~\ref{sec:experiments} are held fixed unless we state a change below.
The figures are multi-panel versions of the same protocol: mean cumulative regret with variability
bands across random seeds, with one panel per setting.

\paragraph{Randomized shift composition.}
The online parameter is drawn with independent coordinates in~$[0.25,0.55]$.
The offline mean is
\(
\theta^\dagger = s\,\theta_* + u,
\)
where~$s\in(0,1]$ and $u$ is uniform on~$[0,c]^d$ with $c\in\{0,0.2,0.4,0.6,0.8\}$.
The pairs~$(s,c)$ are chosen so that as~$c$ increases, the additive offset~$u$ has larger range while the
scale factor~$s$ toward~$\theta_*$ decreases; at $c=0$ one has $s=1$ and $u=0$ (a pure re-scaling
parameterization of the online vector).
Figure~\ref{fig:app-exp-shift} stacks these five misspecification strengths; we plot Ellipsoidal-MINUCB
and the best purely offline policy on the same axis for each panel.
\begin{figure}[h]
  \centering
  \includegraphics[width=0.98\linewidth]{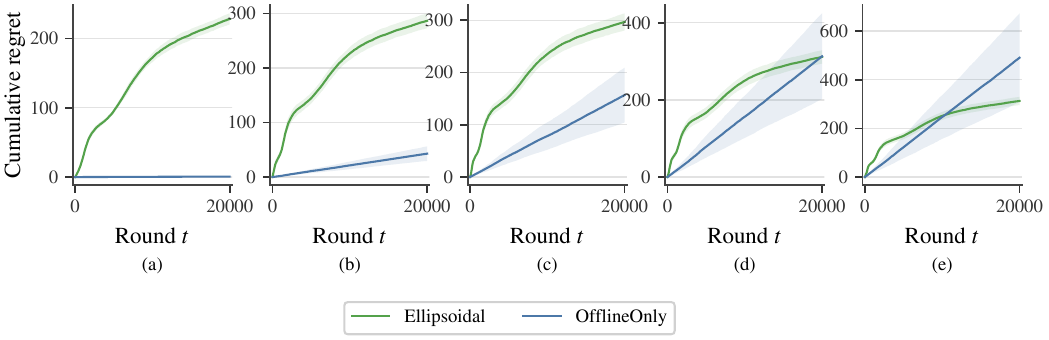}
  \caption{Randomized shift sweep: for each~$c$, mean cumulative regret under the~$(s,u)$ law above
  (left to right, increasing~$c$; five panels in the published figure).}
  \label{fig:app-exp-shift}
\end{figure}

\paragraph{Fixed online parameter, varying offline mean on one coordinate.}
We fix~$\theta_*=(2,1,1,1,1)$ and change only~$\theta^\dagger_1$ among
$\{0,1,2,1,4\}$ (with the remaining coordinates~$1$ in each case, so the middle and fourth panels repeat
the same~$\theta^\dagger$ used as a check on seed noise).
Figure~\ref{fig:app-exp-ablation} compares the full method to two stripped variants: one that only uses
the offline design matrix in the online branch, and one that only uses the online ridge design (no
offline pooling in the same sense as the main text).
\begin{figure}[h]
  \centering
  \includegraphics[width=0.98\linewidth]{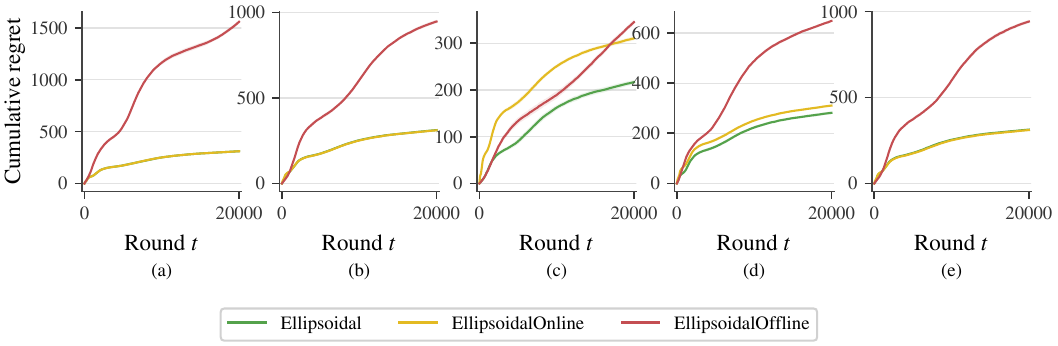}
  \caption{Ablation: five values of~$\theta^\dagger_1$ with~$\theta_*$ as above, same hyperparameters
  otherwise.}
  \label{fig:app-exp-ablation}
\end{figure}

\paragraph{Covariate shift on offline data only.}
The online and offline parameters are generated from the same random law, but offline covariates are
drawn from an axis-aligned box~$\prod_j[\ell_j,h_j]$ inside the support used at play time.
In particular, the first feature uses~$[0,1]$, and coordinates~$2,\ldots,d$ use~$[0,w]$ with~$w$ in a finite
decreasing set that includes $1$, a moderate value, and small values down to~$0.01$.
For small~$w$ the offline design places almost no energy on several directions, so the pooled statistics
in those directions are driven almost entirely by the online data even when~$\theta^\dagger=\theta_*$ on
average.
Figure~\ref{fig:app-exp-div} reports the same algorithm comparison as in Figure~\ref{fig:app-exp-shift}, here indexed by~$w$.
\begin{figure}[h]
  \centering
  \includegraphics[width=0.98\linewidth]{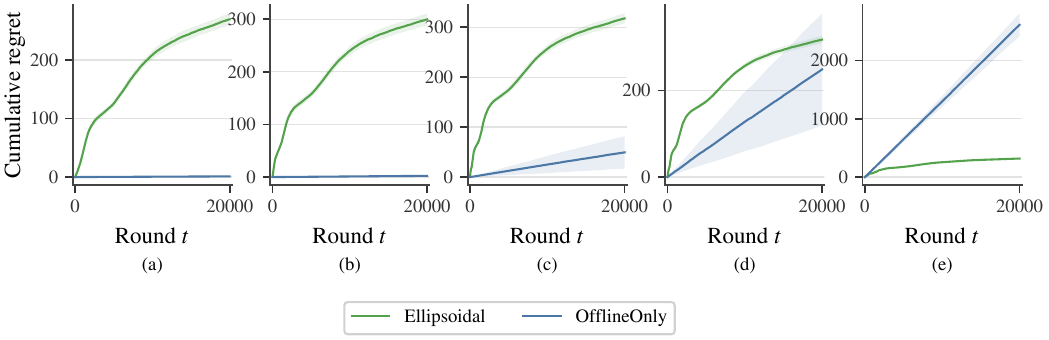}
  \caption{Offline-coverage study: each panel is a value of~$w$ in the family above (narrow
  offline support on several coordinates, wide online support; five panels in the published figure).}
  \label{fig:app-exp-div}
\end{figure}
